# Supplementary material for: Opted Out, Yet Tracked: Are Regulations Enough to Protect Your Privacy?
Source: arXiv:2202.00885 source file (2023-10-06)
Supplement: Supplementary file 1 [file appendix_1.tex]

\begin{table*}
\centering
	\caption{The summary of advertisers/bidders/3rd party service that appeared before opt-out and disappeared after opt-out in HTTP data, part 1}
	\label{tbl:in_train_not_in_test_1}
\begin{tabular}{|l|l|l|l|l|l|l|} 
\hline
\textbf{Advertiser/Bidders/3rd Party Service}        & \textbf{Onetrust\_CA} & \textbf{~Cookiebot\_CA} & \textbf{~Central\_CA} & \textbf{~Onetrust\_GE} & \textbf{~Cookiebot\_GE} & \textbf{~Central\_GE}  \\ 
\hline
\textbf{TrafficJunky}                                & 1                     & 1                       & 1                     & 1                      & 1                       & 1                      \\ 
\hline
\textbf{Streamray}                                   & 1                     & 1                       & 1                     & 1                      & 1                       & 1                      \\ 
\hline
\textbf{Wingify}                                     & 9                     & 9                       & \textcolor{blue}{X}                     & 6                      & 6                       & \textcolor{blue}{X}                      \\ 
\hline
\textbf{iovation}                                    & 1                     & 1                       & 1                     & 2                      & 2                       & 2                      \\ 
\hline
\textbf{SmartAdServer}                               & 5                     & 5                       & \textcolor{blue}{X}                     & 1                      & 2                       & \textcolor{blue}{X}                      \\ 
\hline
\textbf{FriendFinder Networks}                       & 1                     & 1                       & 1                     & 1                      & 1                       & 1                      \\ 
\hline
\textbf{Crazy Egg}                                   & 14                    & 13                      & \textcolor{blue}{X}                     & \textcolor{blue}{X}                      & \textcolor{blue}{X}                       & \textcolor{blue}{X}                      \\ 
\hline
\textbf{Infolinks}                                   & 2                     & 2                       & 2                     & 1                      & 1                       & \textcolor{blue}{X}                      \\ 
\hline
\textbf{TrustX}                                      & 12                    & 11                      & \textcolor{blue}{X}                     & \textcolor{blue}{X}                      & \textcolor{blue}{X}                       & \textcolor{blue}{X}                      \\ 
\hline
\textbf{DoublePimp}                                  & 1                     & 1                       & 1                     & 1                      & 1                       & 1                      \\ 
\hline
\textbf{Renegade Internet}                           & 1                     & \textcolor{blue}{X}                       & \textcolor{blue}{X}                     & \textcolor{blue}{X}                      & \textcolor{blue}{X}                       & \textcolor{blue}{X}                      \\ 
\hline
\textbf{BlogHer}                                     & 5                     & 5                       & 5                     & 5                      & 5                       & 5                      \\ 
\hline
\textbf{Permutive}                                   & 15                    & 15                      & \textcolor{blue}{X}                     & \textcolor{blue}{X}                      & 10                      & \textcolor{blue}{X}                      \\ 
\hline
\textbf{Merkle}                                      & 11                    & \textcolor{blue}{X}                       & \textcolor{blue}{X}                     & \textcolor{blue}{X}                      & \textcolor{blue}{X}                       & \textcolor{blue}{X}                      \\ 
\hline
\textbf{Undertone}                                   & 10                    & \textcolor{blue}{X}                       & 9                     & 6                      & 6                       & 16                     \\ 
\hline
\textbf{Yieldmo}                                     & 4                     & \textcolor{blue}{X}                       & \textcolor{blue}{X}                     & 1                      & \textcolor{blue}{X}                       & 4                      \\ 
\hline
\textbf{Outbrain}                                    & 12                    & 13                      & \textcolor{blue}{X}                     & 8                      & \textcolor{blue}{X}                       & \textcolor{blue}{X}                      \\ 
\hline
\textbf{TRUSTe}                                      & 4                     & 4                       & \textcolor{blue}{X}                     & 12                     & 9                       & \textcolor{blue}{X}                      \\ 
\hline
\textbf{Yandex}                                      & 9                     & 9                       & \textcolor{blue}{X}                     & 8                      & \textcolor{blue}{X}                       & \textcolor{blue}{X}                      \\ 
\hline
\textbf{JuicyAds}                                    & 1                     & 1                       & 1                     & 1                      & 1                       & 1                      \\ 
\hline
\textbf{Cloudflare}                                  & 1                     & 2                       & 2                     & 4                      & 4                       & 4                      \\ 
\hline
\textbf{Pinterest}                                   & 14                    & 14                      & \textcolor{blue}{X}                     & 14                     & 14                      & \textcolor{blue}{X}                      \\ 
\hline
\textbf{ExoClick}                                    & 1                     & 1                       & 1                     & 1                      & 1                       & 1                      \\ 
\hline
\textbf{Stripe}                                      & 6                     & 6                       & \textcolor{blue}{X}                     & 4                      & 3                       & \textcolor{blue}{X}                      \\ 
\hline
\textbf{Adzerk}                                      & 1                     & 1                       & 1                     & 1                      & 1                       & 1                      \\ 
\hline
\textbf{Exosrv}                                      & 1                     & 1                       & 1                     & 1                      & 1                       & 1                      \\ 
\hline
\textbf{ClickDistrict}                               & 6                     & 8                       & 8                     & 2                      & 2                       & \textcolor{blue}{X}                      \\ 
\hline
\textbf{OnAudience}                                  & 14                    & 9                       & 7                     & 5                      & 7                       & 2                      \\ 
\hline
\textbf{Narrative}                                   & 14                    & 12                      & 12                    & \textcolor{blue}{X}                      & \textcolor{blue}{X}                       & \textcolor{blue}{X}                      \\ 
\hline
\textbf{Acxiom}                                      & 15                    & 7                       & 11                    & 1                      & 1                       & 1                      \\ 
\hline
\textbf{C3 Metrics}                                  & 7                     & 3                       & 1                     & \textcolor{blue}{X}                      & \textcolor{blue}{X}                       & \textcolor{blue}{X}                      \\ 
\hline
\textbf{Amplitude}                                   & 12                    & 12                      & 12                    & 9                      & 9                       & 9                      \\ 
\hline
\textbf{Tremor Video}                                & 5                     & \textcolor{blue}{X}                       & \textcolor{blue}{X}                     & \textcolor{blue}{X}                      & 11                      & 9                      \\ 
\hline
\textbf{WPP}                                         & 1                     & 10                      & \textcolor{blue}{X}                     & \textcolor{blue}{X}                      & 6                       & 2                      \\ 
\hline
\textbf{Survata}                                     & 2                     & 12                      & 3                     & \textcolor{blue}{X}                      & 8                       & 9                      \\ 
\hline
\textbf{Optimizely}                                  & 15                    & 14                      & \textcolor{blue}{X}                     & 14                     & 14                      & 14                     \\ 
\hline
\textbf{Effective Measure}                           & 3                     & 2                       & 2                     & \textcolor{blue}{X}                      & \textcolor{blue}{X}                       & \textcolor{blue}{X}                      \\ 
\hline
\textbf{Bouncex}                                     & 14                    & \textcolor{blue}{X}                       & \textcolor{blue}{X}                     & \textcolor{blue}{X}                      & 11                      & \textcolor{blue}{X}                      \\ 
\hline
\textbf{Sourcepoint}                                 & 5                     & 4                       & \textcolor{blue}{X}                     & \textcolor{blue}{X}                      & 2                       & 3                      \\ 
\hline
\textbf{Branch}                                      & 9                     & 9                       & \textcolor{blue}{X}                     & 8                      & 8                       & 7                      \\ 
\hline
\textbf{Rakuten}                                     & 5                     & 4                       & 16                    & 4                      & 4                       & 16                     \\ 
\hline
\textbf{m6d}                                         & 11                    & 9                       & 8                     & 3                      & 3                       & 3                      \\ 
\hline
\textbf{Rambler}                                     & 2                     & 5                       & 3                     & 2                      & 2                       & 2                      \\ 
\hline
\textbf{TNS}                                         & 4                     & 4                       & 1                     & 4                      & 4                       & 2                      \\ 
\hline
\textbf{VKontakte}                                   & 2                     & 2                       & 2                     & 2                      & 2                       & 2                      \\ 
\hline
\textbf{AdFox}                                       & 2                     & 2                       & \textcolor{blue}{X}                     & 2                      & 2                       & \textcolor{blue}{X}                      \\ 
\hline
\textbf{GetIntent}                                   & 4                     & 4                       & 2                     & 1                      & \textcolor{blue}{X}                       & \textcolor{blue}{X}                      \\ 
\hline
\textbf{RuTarget}                                    & 2                     & 2                       & 2                     & 1                      & \textcolor{blue}{X}                       & 1                      \\ 
\hline
\textbf{BetweenDigital}                              & 10                    & 8                       & \textcolor{blue}{X}                     & \textcolor{blue}{X}                      & 2                       & \textcolor{blue}{X}                      \\ 
\hline
\textbf{AdRiver}                                     & 2                     & 2                       & \textcolor{blue}{X}                     & 1                      & \textcolor{blue}{X}                       & \textcolor{blue}{X}                      \\ 
\hline
\textbf{Weborama}                                    & 2                     & 4                       & 12                    & 2                      & 2                       & 13                     \\ 
\hline
\textbf{DataMind.ru}                                 & 2                     & 2                       & 2                     & 1                      & \textcolor{blue}{X}                       & 1                      \\ 
\hline
\textbf{1plusx}                                      & 2                     & 4                       & \textcolor{blue}{X}                     & 1                      & 1                       & \textcolor{blue}{X}                      \\ 
\hline
\textbf{Adelphic}                                    & 2                     & 4                       & 1                     & \textcolor{blue}{X}                      & \textcolor{blue}{X}                       & \textcolor{blue}{X}                      \\ 
\hline
\textbf{EMX}                                         & 6                     & \textcolor{blue}{X}                       & \textcolor{blue}{X}                     & \textcolor{blue}{X}                      & 7                       & \textcolor{blue}{X}                      \\ 
\hline
\textbf{IntimateMerger}                              & 5                     & 4                       & 4                     & 2                      & 1                       & 1                      \\ 
\hline
\textbf{Powerlinks}                                  & 4                     & 3                       & 4                     & \textcolor{blue}{X}                      & \textcolor{blue}{X}                       & \textcolor{blue}{X}                      \\ 
\hline
\textbf{Eyeota}                                      & 10                    & 8                       & \textcolor{blue}{X}                     & 8                      & 7                       & 3                      \\ 
\hline
\textbf{Appier}                                      & 7                     & 7                       & \textcolor{blue}{X}                     & \textcolor{blue}{X}                      & \textcolor{blue}{X}                       & \textcolor{blue}{X}                      \\ 
\hline
\textbf{iPerceptions}                                & 4                     & 4                       & 4                     & 4                      & 4                       & 4                      \\ 
\hline
\textbf{Flashtalking}                                & 4                     & 7                       & \textcolor{blue}{X}                     & 9                      & 8                       & 1                      \\ 
\hline
\textbf{RunAds}                                      & 5                     & 5                       & 4                     & 5                      & 4                       & 4                      \\ 
\hline
\textbf{Adswizz}                                     & 5                     & \textcolor{blue}{X}                       & 3                     & 3                      & 3                       & 3                      \\ 
\hline
\textbf{Research Now}                                & 4                     & 9                       & 1                     & 3                      & 3                       & 3                      \\ 
\hline
\textbf{LiveIntent}                                  & 8                     & \textcolor{blue}{X}                       & \textcolor{blue}{X}                     & \textcolor{blue}{X}                      & \textcolor{blue}{X}                       & \textcolor{blue}{X}                      \\ 
\hline
\textbf{Proclivity}                                  & 5                     & 8                       & 6                     & \textcolor{blue}{X}                      & \textcolor{blue}{X}                       & \textcolor{blue}{X}                      \\ 
\hline
\textbf{Markit}                                      & 3                     & 3                       & 16                    & 2                      & 2                       & 16                    
\\
\hline
\end{tabular}
\end{table*}

\begin{table*}
\centering
	\caption{The summary of advertisers/bidders/3rd party service that appeared before opt-out and disappeared after opt-out in HTTP data, part 2}
	\label{tbl:in_train_not_in_test_2}
\begin{tabular}{|l|l|l|l|l|l|l|} 
\hline
\textbf{Advertiser/Bidders/3rd Party Service}        & \textbf{Onetrust\_CA} & \textbf{~Cookiebot\_CA} & \textbf{~Central\_CA} & \textbf{~Onetrust\_GE} & \textbf{~Cookiebot\_GE} & \textbf{~Central\_GE}  \\ 
\hline
\textbf{mParticle}                                   & 3                     & 3                       & 3                     & 3                      & 3                       & 3                      \\ 
\hline
\textbf{MobileAdTrading}                             & 4                     & 3                       & 1                     & \textcolor{blue}{X}                      & \textcolor{blue}{X}                       & \textcolor{blue}{X}                      \\ 
\hline
\textbf{Adiant}                                      & 4                     & 3                       & 1                     & \textcolor{blue}{X}                      & \textcolor{blue}{X}                       & \textcolor{blue}{X}                      \\ 
\hline
\textbf{Datonics}                                    & 7                     & 6                       & 3                     & 3                      & 3                       & 16                     \\ 
\hline
\textbf{Cross Pixel}                                 & 7                     & 1                       & 13                    & \textcolor{blue}{X}                      & \textcolor{blue}{X}                       & 16                     \\ 
\hline
\textbf{IponWeb}                                     & 8                     & 7                       & 4                     & \textcolor{blue}{X}                      & \textcolor{blue}{X}                       & \textcolor{blue}{X}                      \\ 
\hline
\textbf{Pardot}                                      & 3                     & 3                       & 3                     & 1                      & 1                       & 1                      \\ 
\hline
\textbf{Marketo}                                     & 8                     & 8                       & 8                     & 6                      & 6                       & 6                      \\ 
\hline
\textbf{Datalogix}                                   & 4                     & 4                       & 1                     & 1                      & 1                       & 1                      \\ 
\hline
\textbf{Skimlinks}                                   & 9                     & 8                       & \textcolor{blue}{X}                     & 1                      & \textcolor{blue}{X}                       & 7                      \\ 
\hline
\textbf{CBS Interactive}                             & 4                     & 4                       & 3                     & \textcolor{blue}{X}                      & 1                       & 1                      \\ 
\hline
\textbf{Cedexis}                                     & 5                     & 5                       & 5                     & \textcolor{blue}{X}                      & 5                       & 5                      \\ 
\hline
\textbf{InMobi}                                      & 6                     & 8                       & 1                     & \textcolor{blue}{X}                      & \textcolor{blue}{X}                       & \textcolor{blue}{X}                      \\ 
\hline
\textbf{Keywee}                                      & 4                     & 4                       & \textcolor{blue}{X}                     & \textcolor{blue}{X}                      & 1                       & 2                      \\ 
\hline
\textbf{Gigya}                                       & 7                     & 7                       & \textcolor{blue}{X}                     & 6                      & 6                       & 6                      \\ 
\hline
\textbf{Connatix.com}   & 6                     & 5                       & \textcolor{blue}{X}                     & 2                      & 4                       & \textcolor{blue}{X}                      \\ 
\hline
\textbf{BidTheatre}                                  & 8                     & 5                       & \textcolor{blue}{X}                     & 4                      & 1                       & 2                      \\ 
\hline
\textbf{Connexity}                                   & 5                     & 4                       & 4                     & \textcolor{blue}{X}                      & \textcolor{blue}{X}                       & \textcolor{blue}{X}                      \\ 
\hline
\textbf{ClickTale}                                   & 9                     & 8                       & 9                     & 5                      & 4                       & 4                      \\ 
\hline
\textbf{Awin}                                        & 7                     & 7                       & 7                     & 6                      & 7                       & 4                      \\ 
\hline
\textbf{Compuware}                                   & 3                     & 3                       & 3                     & 3                      & 3                       & 3                      \\ 
\hline
\textbf{LivePerson}                                  & 7                     & 7                       & 6                     & 5                      & 5                       & 5                      \\ 
\hline
\textbf{Affinity}                                    & 1                     & 1                       & 1                     & 1                      & 1                       & 1                      \\ 
\hline
\textbf{Intergi}                                     & 3                     & 3                       & 3                     & 2                      & 2                       & 2                      \\ 
\hline
\textbf{Caraytech}                                   & 4                     & 3                       & \textcolor{blue}{X}                     & 1                      & 1                       & 1                      \\ 
\hline
\textbf{Adara Media}                                 & 5                     & 4                       & 3                     & 2                      & 2                       & 2                      \\ 
\hline
\textbf{reddit}                                      & 11                    & 11                      & \textcolor{blue}{X}                     & 8                      & 8                       & \textcolor{blue}{X}                      \\ 
\hline
\textbf{RichAudience}                                & 2                     & 5                       & \textcolor{blue}{X}                     & 1                      & 2                       & \textcolor{blue}{X}                      \\ 
\hline
\textbf{Paypal}                                      & 3                     & 3                       & 3                     & 3                      & 3                       & 3                      \\ 
\hline
\textbf{Segment.io}         & 7                     & 7                       & \textcolor{blue}{X}                     & \textcolor{blue}{X}                      & 7                       & \textcolor{blue}{X}                      \\ 
\hline
\textbf{SiftScience}                                 & 4                     & 4                       & 1                     & 3                      & 3                       & \textcolor{blue}{X}                      \\ 
\hline
\textbf{Jivox}                                       & 5                     & 5                       & 2                     & 3                      & 3                       & 3                      \\ 
\hline
\textbf{Forbes}                                      & 2                     & 2                       & 2                     & 2                      & 2                       & 2                      \\ 
\hline
\textbf{MaxPoint}                                    & 5                     & 7                       & 9                     & \textcolor{blue}{X}                      & \textcolor{blue}{X}                       & \textcolor{blue}{X}                      \\ 
\hline
\textbf{AvidMedia}                                   & 3                     & 2                       & \textcolor{blue}{X}                     & \textcolor{blue}{X}                      & \textcolor{blue}{X}                       & \textcolor{blue}{X}                      \\ 
\hline
\textbf{dianomi}                                     & 3                     & 3                       & 3                     & 2                      & 2                       & 2                      \\ 
\hline
\textbf{Netmining}                                   & 2                     & 1                       & 1                     & 3                      & 1                       & 2                      \\ 
\hline
\textbf{Limelight Networks}                          & 9                     & 9                       & 9                     & 7                      & 8                       & 7                      \\ 
\hline
\textbf{TouchCommerce}                               & 3                     & 3                       & 3                     & 3                      & 3                       & 3                      \\ 
\hline
\textbf{Demandbase}                                  & 4                     & 4                       & 4                     & 5                      & 5                       & 5                      \\ 
\hline
\textbf{VINDICO}                                     & 7                     & 6                       & 14                    & 6                      & 6                       & 16                     \\ 
\hline
\textbf{Webtrekk}                                    & 1                     & 1                       & 1                     & 1                      & 1                       & 1                      \\ 
\hline
\textbf{Baynote}                                     & 2                     & 2                       & 1                     & 2                      & 2                       & 2                      \\ 
\hline
\textbf{Avocet}                                      & 3                     & 5                       & 5                     & 3                      & 1                       & 1                      \\ 
\hline
\textbf{Interpolls}                                  & 2                     & \textcolor{blue}{X}                       & \textcolor{blue}{X}                     & \textcolor{blue}{X}                      & \textcolor{blue}{X}                       & \textcolor{blue}{X}                      \\ 
\hline
\textbf{Adloox}                                      & 2                     & 1                       & \textcolor{blue}{X}                     & 1                      & 1                       & 1                      \\ 
\hline
\textbf{Protected Media}                             & 2                     & 1                       & 2                     & 1                      & 1                       & 1                      \\ 
\hline
\textbf{Primis}                                      & 2                     & 2                       & 2                     & \textcolor{blue}{X}                      & \textcolor{blue}{X}                       & \textcolor{blue}{X}                      \\ 
\hline
\textbf{Mouseflow}                                   & 6                     & 6                       & \textcolor{blue}{X}                     & 3                      & 3                       & \textcolor{blue}{X}                      \\ 
\hline
\textbf{Resonate}                                    & 9                     & 8                       & 2                     & 4                      & 3                       & 4                      \\ 
\hline
\textbf{JustPremium}                                 & 5                     & 8                       & 7                     & \textcolor{blue}{X}                      & 5                       & 4                      \\ 
\hline
\textbf{4INFO}                                       & 5                     & 11                      & 1                     & 2                      & 2                       & 16                     \\ 
\hline
\textbf{Oracle}                                      & 6                     & 5                       & 6                     & 6                      & 6                       & 6                      \\ 
\hline
\textbf{Ensighten}                                   & 8                     & 8                       & \textcolor{blue}{X}                     & 9                      & 9                       & \textcolor{blue}{X}                      \\ 
\hline
\textbf{OnlineMetrix}                                & 3                     & 3                       & 2                     & 2                      & 2                       & 2                      \\ 
\hline
\textbf{Bazaarvoice}                                 & 2                     & 2                       & 2                     & 1                      & 1                       & 1                      \\ 
\hline
\textbf{LiveRamp}                                    & 4                     & 8                       & \textcolor{blue}{X}                     & 5                      & 4                       & \textcolor{blue}{X}                      \\ 
\hline
\textbf{Navegg}                                      & 1                     & 2                       & \textcolor{blue}{X}                     & \textcolor{blue}{X}                      & \textcolor{blue}{X}                       & \textcolor{blue}{X}                      \\ 
\hline
\textbf{TheTimesGroup}                               & 4                     & 4                       & \textcolor{blue}{X}                     & 4                      & 4                       & \textcolor{blue}{X}                      \\ 
\hline
\textbf{Neustar}                                     & 1                     & 1                       & \textcolor{blue}{X}                     & \textcolor{blue}{X}                      & \textcolor{blue}{X}                       & \textcolor{blue}{X}                      \\ 
\hline
\textbf{adscale}                                     & 1                     & 2                       & \textcolor{blue}{X}                     & 3                      & 2                       & \textcolor{blue}{X}                      \\ 
\hline
\textbf{Admeta}                                      & 2                     & \textcolor{blue}{X}                       & 3                     & \textcolor{blue}{X}                      & \textcolor{blue}{X}                       & \textcolor{blue}{X}                      \\ 
\hline
\textbf{AdRoll}                                      & 6                     & 6                       & 12                    & 1                      & 3                       & 16                     \\ 
\hline
\textbf{aidata}                                      & 1                     & 1                       & \textcolor{blue}{X}                     & \textcolor{blue}{X}                      & \textcolor{blue}{X}                       & \textcolor{blue}{X}                      \\ 
\hline
\textbf{Opera}                                       & 1                     & 4                       & \textcolor{blue}{X}                     & 4                      & 3                       & \textcolor{blue}{X}                      \\ 
\hline
\textbf{Bizo}                                        & 1                     & 1                       & 1                     & \textcolor{blue}{X}                      & \textcolor{blue}{X}                       & \textcolor{blue}{X}                      \\ 
\hline
\textbf{Automattic}                                  & 3                     & 3                       & 3                     & 3                      & 3                       & 3                      \\ 
\hline
\textbf{GitHub}                                      & 1                     & 1                       & 1                     & 1                      & 1                       & 1                      \\ 
\hline
\end{tabular}
\end{table*}

\begin{table*}
\centering
	\caption{The summary of advertisers/bidders/3rd party service that appeared before opt-out and disappeared after opt-out in HTTP data, part 3}
	\label{tbl:in_train_not_in_test_3}
\begin{tabular}{|l|l|l|l|l|l|l|} 
\hline
\textbf{Advertiser/Bidders/3rd Party Service}        & \textbf{Onetrust\_CA} & \textbf{~Cookiebot\_CA} & \textbf{~Central\_CA} & \textbf{~Onetrust\_GE} & \textbf{~Cookiebot\_GE} & \textbf{~Central\_GE}  \\ 
\hline
\textbf{IAB}                                         & 1                     & 1                       & 1                     & \textcolor{blue}{X}                      & \textcolor{blue}{X}                       & \textcolor{blue}{X}                      \\ 
\hline
\textbf{SteelHouse}                                  & 4                     & 4                       & 16                    & 3                      & 3                       & 16                     \\ 
\hline
\textbf{MailChimp}                                   & 2                     & 2                       & \textcolor{blue}{X}                     & \textcolor{blue}{X}                      & 2                       & \textcolor{blue}{X}                      \\ 
\hline
\textbf{rtk}                                         & 1                     & 1                       & 1                     & 1                      & 1                       & 1                      \\ 
\hline
\textbf{ucfunnel}                                    & 1                     & 6                       & \textcolor{blue}{X}                     & \textcolor{blue}{X}                      & \textcolor{blue}{X}                       & \textcolor{blue}{X}                      \\ 
\hline
\textbf{Vimeo}                                       & 3                     & 3                       & 3                     & 4                      & 3                       & 3                      \\ 
\hline
\textbf{AppsFlyer}                                   & 2                     & 2                       & 2                     & 2                      & 2                       & 2                      \\ 
\hline
\textbf{MaxMind}                                     & 1                     & 1                       & 1                     & 1                      & 1                       & 1                      \\ 
\hline
\textbf{Go Daddy}                                    & 1                     & 1                       & 1                     & 1                      & 1                       & 1                      \\ 
\hline
\textbf{Smartlook}                                   & 2                     & 2                       & 2                     & 2                      & 2                       & 2                      \\ 
\hline
\textbf{GetSiteControl}                              & 2                     & 2                       & 2                     & 2                      & 2                       & 2                      \\ 
\hline
\textbf{Trafmag}                                     & 2                     & 1                       & \textcolor{blue}{X}                     & \textcolor{blue}{X}                      & \textcolor{blue}{X}                       & \textcolor{blue}{X}                      \\ 
\hline
\textbf{AdvancedStore}                               & 6                     & 9                       & 12                    & \textcolor{blue}{X}                      & \textcolor{blue}{X}                       & 1                      \\ 
\hline
\textbf{BrightRoll}                                  & 1                     & 1                       & 1                     & \textcolor{blue}{X}                      & \textcolor{blue}{X}                       & \textcolor{blue}{X}                      \\ 
\hline
\textbf{InsightExpress}                              & 11                    & 6                       & \textcolor{blue}{X}                     & 2                      & 3                       & 1                      \\ 
\hline
\textbf{AdKernel}                                    & 7                     & 8                       & 9                     & 1                      & 1                       & \textcolor{blue}{X}                      \\ 
\hline
\textbf{LKQD}                                        & 7                     & 6                       & 2                     & 1                      & \textcolor{blue}{X}                       & 1                      \\ 
\hline
\textbf{Bidtellect}                                  & 4                     & 3                       & \textcolor{blue}{X}                     & 1                      & \textcolor{blue}{X}                       & \textcolor{blue}{X}                      \\ 
\hline
\textbf{FuturePlc}                                   & 3                     & 3                       & 3                     & 4                      & 3                       & 3                      \\ 
\hline
\textbf{EQ Ads}                                      & 3                     & 3                       & 6                     & \textcolor{blue}{X}                      & \textcolor{blue}{X}                       & 1                      \\ 
\hline
\textbf{Itch}                                        & 1                     & 1                       & 1                     & 1                      & 1                       & 1                      \\ 
\hline
\textbf{Publishers Clearing House}                   & 1                     & 1                       & 1                     & 1                      & 1                       & 1                      \\ 
\hline
\textbf{Sublime Skinz}                               & 2                     & 2                       & 2                     & 1                      & 1                       & 1                      \\ 
\hline
\textbf{CPMStar}                                     & 1                     & 1                       & 1                     & 1                      & 1                       & 1                      \\ 
\hline
\textbf{Venatus Media}                               & 1                     & 1                       & 1                     & \textcolor{blue}{X}                      & \textcolor{blue}{X}                       & \textcolor{blue}{X}                      \\ 
\hline
\textbf{Traverse}                                    & 1                     & 1                       & 1                     & \textcolor{blue}{X}                      & \textcolor{blue}{X}                       & \textcolor{blue}{X}                      \\ 
\hline
\textbf{BlueCava}                                    & 4                     & 3                       & 1                     & 1                      & 1                       & 1                      \\ 
\hline
\textbf{Storygize}                                   & 5                     & 6                       & 1                     & 1                      & 1                       & \textcolor{blue}{X}                      \\ 
\hline
\textbf{iBehavior}                                   & 4                     & 11                      & 1                     & 6                      & 7                       & 1                      \\ 
\hline
\textbf{Sojern}                                      & 3                     & 3                       & 3                     & 2                      & 2                       & 2                      \\ 
\hline
\textbf{Kenshoo}                                     & 6                     & 6                       & 6                     & 5                      & 5                       & 5                      \\ 
\hline
\textbf{PebblePost}                                  & 2                     & 2                       & 2                     & 1                      & 1                       & 1                      \\ 
\hline
\textbf{SessionCam}                                  & 1                     & \textcolor{blue}{X}                       & 1                     & 1                      & 1                       & 1                      \\ 
\hline
\textbf{Selectable Media}                            & 2                     & 2                       & \textcolor{blue}{X}                     & \textcolor{blue}{X}                      & \textcolor{blue}{X}                       & \textcolor{blue}{X}                      \\ 
\hline
\textbf{AuditedMedia}                                & 2                     & 2                       & \textcolor{blue}{X}                     & \textcolor{blue}{X}                      & 2                       & \textcolor{blue}{X}                      \\ 
\hline
\textbf{Bombora}                                     & 3                     & 11                      & \textcolor{blue}{X}                     & 6                      & 6                       & 6                      \\ 
\hline
\textbf{ShareThis}                                   & 5                     & 4                       & 8                     & 2                      & 3                       & 16                     \\ 
\hline
\textbf{FundraiseUp}                                 & 1                     & 1                       & 1                     & 1                      & 1                       & 1                      \\ 
\hline
\textbf{LuckyOrange}                                 & 1                     & 1                       & 1                     & \textcolor{blue}{X}                      & \textcolor{blue}{X}                       & 1                      \\ 
\hline
\textbf{Adjust}                                      & 1                     & 1                       & 1                     & 1                      & 1                       & 1                      \\ 
\hline
\textbf{Think Realtime}                              & 1                     & 1                       & 1                     & 1                      & 1                       & 1                      \\ 
\hline
\textbf{The Heron Partnership}                       & 1                     & 1                       & 1                     & 1                      & 1                       & 1                      \\ 
\hline
\textbf{Monetate}                                    & 2                     & 2                       & 2                     & 2                      & 2                       & 2                      \\ 
\hline
\textbf{NextPerformance}                             & 2                     & 1                       & 16                    & 2                      & 2                       & 16                     \\ 
\hline
\textbf{mediaFORGE}                                  & 2                     & \textcolor{blue}{X}                       & 16                    & 1                      & 1                       & 16                     \\ 
\hline
\textbf{DC Storm}                                    & 2                     & \textcolor{blue}{X}                       & 1                     & \textcolor{blue}{X}                      & \textcolor{blue}{X}                       & \textcolor{blue}{X}                      \\ 
\hline
\textbf{Sortable}                                    & 3                     & 3                       & 3                     & \textcolor{blue}{X}                      & 3                       & 3                      \\ 
\hline
\textbf{VigLink}                                     & 3                     & 4                       & 3                     & 1                      & 1                       & 1                      \\ 
\hline
\textbf{NetShelter}                                  & 1                     & 1                       & 1                     & \textcolor{blue}{X}                      & \textcolor{blue}{X}                       & \textcolor{blue}{X}                      \\ 
\hline
\textbf{Teads.tv}       & 3                     & \textcolor{blue}{X}                       & \textcolor{blue}{X}                     & 1                      & 9                       & \textcolor{blue}{X}                      \\ 
\hline
\textbf{Yieldify}                                    & 2                     & 2                       & 2                     & 2                      & 2                       & 2                      \\ 
\hline
\textbf{Fullstory}                                   & 3                     & 3                       & 4                     & 2                      & 2                       & 2                      \\ 
\hline
\textbf{BuySellAds}                                  & 2                     & 2                       & \textcolor{blue}{X}                     & 2                      & 2                       & \textcolor{blue}{X}                      \\ 
\hline
\textbf{Tinder}                                      & 1                     & 1                       & \textcolor{blue}{X}                     & 1                      & 1                       & \textcolor{blue}{X}                      \\ 
\hline
\textbf{Grapeshot}                                   & 1                     & 1                       & \textcolor{blue}{X}                     & 1                      & 1                       & 1                      \\ 
\hline
\textbf{Browser-Update.org} & 1                     & 2                       & 1                     & 1                      & 1                       & 1                      \\ 
\hline
\textbf{PageFair}                                    & 1                     & 1                       & 1                     & 1                      & 1                       & 1                      \\ 
\hline
\textbf{LockerDome}                                  & 1                     & 2                       & \textcolor{blue}{X}                     & 1                      & 1                       & \textcolor{blue}{X}                      \\ 
\hline
\textbf{HubSpot}                                     & 4                     & 4                       & 4                     & 3                      & 3                       & 3                      \\ 
\hline
\textbf{Pictela}                                     & 2                     & \textcolor{blue}{X}                       & \textcolor{blue}{X}                     & \textcolor{blue}{X}                      & \textcolor{blue}{X}                       & \textcolor{blue}{X}                      \\ 
\hline
\textbf{DistrictM}                                   & 2                     & \textcolor{blue}{X}                       & \textcolor{blue}{X}                     & \textcolor{blue}{X}                      & 1                       & \textcolor{blue}{X}                      \\ 
\hline
\textbf{engage:BDR}                                  & 2                     & 11                      & \textcolor{blue}{X}                     & 3                      & 2                       & \textcolor{blue}{X}                      \\ 
\hline
\textbf{BuzzFeed}                                    & 1                     & 1                       & 1                     & 1                      & 1                       & 1                      \\ 
\hline
\textbf{eBay}                                        & 5                     & 3                       & 2                     & \textcolor{blue}{X}                      & 2                       & 2                      \\ 
\hline
\textbf{CNZZ}                                        & 1                     & 1                       & 1                     & 1                      & 1                       & 1                      \\ 
\hline
\textbf{AT Internet}                                 & 1                     & 1                       & \textcolor{blue}{X}                     & 1                      & 1                       & \textcolor{blue}{X}                      \\ 
\hline
\end{tabular}
\end{table*}

\begin{table*}
\centering
	\caption{The summary of advertisers/bidders/3rd party service that appeared before opt-out and disappeared after opt-out in HTTP data, part 4}
	\label{tbl:in_train_not_in_test_4}
\begin{tabular}{|l|l|l|l|l|l|l|} 
\hline
\textbf{Advertiser/Bidders/3rd Party Service}        & \textbf{Onetrust\_CA} & \textbf{~Cookiebot\_CA} & \textbf{~Central\_CA} & \textbf{~Onetrust\_GE} & \textbf{~Cookiebot\_GE} & \textbf{~Central\_GE}  \\ 
\hline
\textbf{ZEDO}                                        & 1                     & 1                       & 1                     & \textcolor{blue}{X}                      & \textcolor{blue}{X}                       & \textcolor{blue}{X}                      \\ 
\hline
\textbf{AndBeyond}                                   & 1                     & 1                       & 1                     & 1                      & 1                       & 1                      \\ 
\hline
\textbf{RevContent}                                  & 2                     & 4                       & \textcolor{blue}{X}                     & 3                      & 4                       & \textcolor{blue}{X}                      \\ 
\hline
\textbf{OwnPage}                                     & 1                     & \textcolor{blue}{X}                       & 1                     & \textcolor{blue}{X}                      & \textcolor{blue}{X}                       & \textcolor{blue}{X}                      \\ 
\hline
\textbf{Mixpanel}                                    & 3                     & 3                       & 3                     & 3                      & 3                       & 3                      \\ 
\hline
\textbf{ClickTripz}                                  & 1                     & 1                       & 1                     & 1                      & 1                       & 1                      \\ 
\hline
\textbf{Onclusive}                                   & 2                     & 2                       & 2                     & 1                      & 1                       & 1                      \\ 
\hline
\textbf{GumGum}                                      & 1                     & 8                       & \textcolor{blue}{X}                     & 6                      & 2                       & \textcolor{blue}{X}                      \\ 
\hline
\textbf{Gravity}                                     & 1                     & 1                       & \textcolor{blue}{X}                     & \textcolor{blue}{X}                      & 1                       & \textcolor{blue}{X}                      \\ 
\hline
\textbf{Carambola}                                   & 1                     & 1                       & 1                     & \textcolor{blue}{X}                      & \textcolor{blue}{X}                       & \textcolor{blue}{X}                      \\ 
\hline
\textbf{AdGear}                                      & 2                     & 5                       & \textcolor{blue}{X}                     & \textcolor{blue}{X}                      & \textcolor{blue}{X}                       & 2                      \\ 
\hline
\textbf{Kaltura}                                     & 1                     & 1                       & 1                     & 1                      & 1                       & 1                      \\ 
\hline
\textbf{Qualaroo}                                    & 3                     & 3                       & 3                     & 2                      & 2                       & 2                      \\ 
\hline
\textbf{DigitalAdConsortium}                         & 1                     & 1                       & \textcolor{blue}{X}                     & 1                      & 1                       & \textcolor{blue}{X}                      \\ 
\hline
\textbf{AdYouLike}                                   & 2                     & 3                       & \textcolor{blue}{X}                     & 3                      & 2                       & \textcolor{blue}{X}                      \\ 
\hline
\textbf{LiveInternet}                                & 1                     & 1                       & \textcolor{blue}{X}                     & 1                      & 1                       & \textcolor{blue}{X}                      \\ 
\hline
\textbf{BrightTag}                                   & 2                     & 4                       & \textcolor{blue}{X}                     & 4                      & \textcolor{blue}{X}                       & \textcolor{blue}{X}                      \\ 
\hline
\textbf{HP}                                          & 1                     & 1                       & \textcolor{blue}{X}                     & 1                      & 1                       & 1                      \\ 
\hline
\textbf{Curalate}                                    & 2                     & 3                       & 3                     & 3                      & 2                       & 3                      \\ 
\hline
\textbf{GENIEE}                                      & 1                     & \textcolor{blue}{X}                       & \textcolor{blue}{X}                     & 1                      & 1                       & 1                      \\ 
\hline
\textbf{Polar Mobile}                                & 1                     & 1                       & 1                     & \textcolor{blue}{X}                      & \textcolor{blue}{X}                       & \textcolor{blue}{X}                      \\ 
\hline
\textbf{Wayfair}                                     & 1                     & 1                       & 1                     & 1                      & 1                       & 1                      \\ 
\hline
\textbf{ToneMedia}                                   & 1                     & 1                       & 1                     & \textcolor{blue}{X}                      & \textcolor{blue}{X}                       & \textcolor{blue}{X}                      \\ 
\hline
\textbf{BloomReach}                                  & 1                     & 1                       & 1                     & 1                      & 1                       & 1                      \\ 
\hline
\textbf{Certona}                                     & 1                     & 1                       & 1                     & 1                      & 1                       & 1                      \\ 
\hline
\textbf{LoopMe}                                      & 1                     & 1                       & 1                     & 1                      & 1                       & 1                      \\ 
\hline
\textbf{Intent Media}                                & 1                     & 1                       & 1                     & 1                      & 1                       & 1                      \\ 
\hline
\textbf{ChannelAdvisor}                              & 1                     & \textcolor{blue}{X}                       & \textcolor{blue}{X}                     & 1                      & 1                       & 1                      \\ 
\hline
\textbf{DynamicYield}                                & 1                     & 1                       & 1                     & 1                      & 1                       & 1                      \\ 
\hline
\textbf{TurnTo}                                      & 1                     & 1                       & 1                     & \textcolor{blue}{X}                      & \textcolor{blue}{X}                       & \textcolor{blue}{X}                      \\ 
\hline
\textbf{McAfee}                                      & 1                     & 1                       & 1                     & 1                      & 1                       & 1                      \\ 
\hline
\textbf{User Local}                                  & 1                     & 1                       & \textcolor{blue}{X}                     & 1                      & 1                       & \textcolor{blue}{X}                      \\ 
\hline
\textbf{Unruly}                                      & 2                     & 4                       & \textcolor{blue}{X}                     & 2                      & 6                       & \textcolor{blue}{X}                      \\ 
\hline
\textbf{Match.com}       & 1                     & 1                       & 1                     & 1                      & 1                       & 1                      \\ 
\hline
\textbf{Digg}                                        & 1                     & 1                       & 1                     & 1                      & 1                       & 1                      \\ 
\hline
\textbf{Betgenius}                                   & 2                     & 2                       & \textcolor{blue}{X}                     & 1                      & 1                       & 1                      \\ 
\hline
\textbf{Complex Media}                               & 1                     & 1                       & 1                     & 1                      & 1                       & 1                      \\ 
\hline
\textbf{UserVoice}                                   & 1                     & 1                       & 1                     & 1                      & 1                       & 1                      \\ 
\hline
\textbf{StackAdapt}                                  & 1                     & 3                       & \textcolor{blue}{X}                     & 1                      & \textcolor{blue}{X}                       & \textcolor{blue}{X}                      \\ 
\hline
\textbf{Peer39}                                      & 1                     & 1                       & 1                     & 1                      & 1                       & 1                      \\ 
\hline
\textbf{Web.com}          & 1                     & 1                       & \textcolor{blue}{X}                     & 1                      & 1                       & \textcolor{blue}{X}                      \\ 
\hline
\textbf{Evolve}                                      & 1                     & 1                       & 1                     & 1                      & 1                       & 1                      \\ 
\hline
\textbf{MarkMonitor}                                 & 1                     & 1                       & 1                     & 1                      & 1                       & 1                      \\ 
\hline
\textbf{Taleria}                                     & 1                     & 1                       & 1                     & \textcolor{blue}{X}                      & \textcolor{blue}{X}                       & \textcolor{blue}{X}                      \\ 
\hline
\textbf{Underdog Media}                              & 1                     & 1                       & 1                     & 1                      & 1                       & 1                      \\ 
\hline
\textbf{Histats}                                     & 1                     & 1                       & 1                     & 1                      & 1                       & 1                      \\ 
\hline
\textbf{Sunmedia}                                    & 1                     & 1                       & 1                     & 1                      & 1                       & 1                      \\ 
\hline
\textbf{New Relic}                                   & \textcolor{blue}{X}                     & 16                      & \textcolor{blue}{X}                     & \textcolor{blue}{X}                      & 16                      & \textcolor{blue}{X}                      \\ 
\hline
\textbf{Hotjar}                                      & \textcolor{blue}{X}                     & 16                      & \textcolor{blue}{X}                     & \textcolor{blue}{X}                      & 16                      & \textcolor{blue}{X}                      \\ 
\hline
\textbf{Fluct}                                       & \textcolor{blue}{X}                     & 10                      & 4                     & 1                      & \textcolor{blue}{X}                       & \textcolor{blue}{X}                      \\ 
\hline
\textbf{AddThis}                                     & \textcolor{blue}{X}                     & 6                       & \textcolor{blue}{X}                     & \textcolor{blue}{X}                      & 4                       & \textcolor{blue}{X}                      \\ 
\hline
\textbf{Salesforce.com}    & \textcolor{blue}{X}                     & 14                      & \textcolor{blue}{X}                     & \textcolor{blue}{X}                      & 13                      & \textcolor{blue}{X}                      \\ 
\hline
\textbf{Twitter}                                     & \textcolor{blue}{X}                     & 15                      & \textcolor{blue}{X}                     & \textcolor{blue}{X}                      & \textcolor{blue}{X}                       & \textcolor{blue}{X}                      \\ 
\hline
\textbf{Nielsen}                                     & \textcolor{blue}{X}                     & 10                      & \textcolor{blue}{X}                     & \textcolor{blue}{X}                      & 7                       & \textcolor{blue}{X}                      \\ 
\hline
\textbf{Krux}                                        & \textcolor{blue}{X}                     & 4                       & \textcolor{blue}{X}                     & \textcolor{blue}{X}                      & 7                       & \textcolor{blue}{X}                      \\ 
\hline
\textbf{eXelate}                                     & \textcolor{blue}{X}                     & 5                       & \textcolor{blue}{X}                     & \textcolor{blue}{X}                      & 1                       & 3                      \\ 
\hline
\textbf{Improve Digital}                             & \textcolor{blue}{X}                     & 1                       & \textcolor{blue}{X}                     & 2                      & 8                       & \textcolor{blue}{X}                      \\ 
\hline
\textbf{Tealium}                                     & \textcolor{blue}{X}                     & 10                      & 9                     & \textcolor{blue}{X}                      & 6                       & 5                      \\ 
\hline
\textbf{Akamai}                                      & \textcolor{blue}{X}                     & 15                      & \textcolor{blue}{X}                     & \textcolor{blue}{X}                      & 15                      & \textcolor{blue}{X}                      \\ 
\hline
\textbf{VDX}                                         & \textcolor{blue}{X}                     & 1                       & \textcolor{blue}{X}                     & \textcolor{blue}{X}                      & \textcolor{blue}{X}                       & \textcolor{blue}{X}                      \\ 
\hline
\textbf{DataXu}                                      & \textcolor{blue}{X}                     & 4                       & \textcolor{blue}{X}                     & \textcolor{blue}{X}                      & \textcolor{blue}{X}                       & \textcolor{blue}{X}                      \\ 
\hline
\textbf{Technorati}                                  & \textcolor{blue}{X}                     & 12                      & \textcolor{blue}{X}                     & 3                      & 5                       & \textcolor{blue}{X}                      \\ 
\hline
\textbf{DG}                                          & \textcolor{blue}{X}                     & 8                       & \textcolor{blue}{X}                     & 3                      & 13                      & 11                     \\ 
\hline
\textbf{cXense}                                      & \textcolor{blue}{X}                     & 6                       & 5                     & \textcolor{blue}{X}                      & 6                       & 6                      \\ 
\hline
\textbf{Sonobi}                                      & \textcolor{blue}{X}                     & 1                       & \textcolor{blue}{X}                     & \textcolor{blue}{X}                      & 1                       & \textcolor{blue}{X}                      \\ 
\hline
\textbf{Commission Junction}                         & \textcolor{blue}{X}                     & 1                       & \textcolor{blue}{X}                     & \textcolor{blue}{X}                      & \textcolor{blue}{X}                       & \textcolor{blue}{X}                      \\ 
\hline
\textbf{media.net}       & \textcolor{blue}{X}                     & 5                       & \textcolor{blue}{X}                     & \textcolor{blue}{X}                      & 1                       & \textcolor{blue}{X}                      \\ 
\hline
\end{tabular}
\end{table*}

\begin{table*}
\centering
	\caption{The summary of advertisers/bidders/3rd party service that appeared before opt-out and disappeared after opt-out in HTTP data, part 5}
	\label{tbl:in_train_not_in_test_5}
\begin{tabular}{|l|l|l|l|l|l|l|} 
\hline
\textbf{Advertiser/Bidders/3rd Party Service}        & \textbf{Onetrust\_CA} & \textbf{~Cookiebot\_CA} & \textbf{~Central\_CA} & \textbf{~Onetrust\_GE} & \textbf{~Cookiebot\_GE} & \textbf{~Central\_GE}  \\ 
\hline
\textbf{Parse.ly}        & \textcolor{blue}{X}                     & 10                      & \textcolor{blue}{X}                     & \textcolor{blue}{X}                      & \textcolor{blue}{X}                       & 8                      \\ 
\hline
\textbf{DoubleVerify}                                & \textcolor{blue}{X}                     & 11                      & \textcolor{blue}{X}                     & 5                      & 6                       & 1                      \\ 
\hline
\textbf{TubeMogul}                                   & \textcolor{blue}{X}                     & 6                       & 2                     & 2                      & 2                       & 2                      \\ 
\hline
\textbf{Microsoft}                                   & \textcolor{blue}{X}                     & 13                      & \textcolor{blue}{X}                     & \textcolor{blue}{X}                      & 16                      & \textcolor{blue}{X}                      \\ 
\hline
\textbf{Moat}                                        & \textcolor{blue}{X}                     & 1                       & \textcolor{blue}{X}                     & \textcolor{blue}{X}                      & 7                       & \textcolor{blue}{X}                      \\ 
\hline
\textbf{LinkedIn}                                    & \textcolor{blue}{X}                     & 11                      & \textcolor{blue}{X}                     & \textcolor{blue}{X}                      & 14                      & \textcolor{blue}{X}                      \\ 
\hline
\textbf{Yieldlab}                                    & \textcolor{blue}{X}                     & 5                       & 3                     & \textcolor{blue}{X}                      & 5                       & 2                      \\ 
\hline
\textbf{FreeWheel}                                   & \textcolor{blue}{X}                     & 3                       & \textcolor{blue}{X}                     & 8                      & 2                       & \textcolor{blue}{X}                      \\ 
\hline
\textbf{Semasio}                                     & \textcolor{blue}{X}                     & 12                      & 7                     & 1                      & 3                       & 2                      \\ 
\hline
\textbf{Brightcove}                                  & \textcolor{blue}{X}                     & 9                       & \textcolor{blue}{X}                     & 4                      & 10                      & \textcolor{blue}{X}                      \\ 
\hline
\textbf{Adform}                                      & \textcolor{blue}{X}                     & 1                       & \textcolor{blue}{X}                     & \textcolor{blue}{X}                      & \textcolor{blue}{X}                       & \textcolor{blue}{X}                      \\ 
\hline
\textbf{Simpli.fi}       & \textcolor{blue}{X}                     & 3                       & \textcolor{blue}{X}                     & \textcolor{blue}{X}                      & \textcolor{blue}{X}                       & \textcolor{blue}{X}                      \\ 
\hline
\textbf{Drawbridge}                                  & \textcolor{blue}{X}                     & 1                       & \textcolor{blue}{X}                     & \textcolor{blue}{X}                      & \textcolor{blue}{X}                       & \textcolor{blue}{X}                      \\ 
\hline
\textbf{Adality}                                     & \textcolor{blue}{X}                     & 2                       & 2                     & 1                      & 2                       & 1                      \\ 
\hline
\textbf{ADITION}                                     & \textcolor{blue}{X}                     & 5                       & \textcolor{blue}{X}                     & 1                      & \textcolor{blue}{X}                       & \textcolor{blue}{X}                      \\ 
\hline
\textbf{SpringServe}                                 & \textcolor{blue}{X}                     & 2                       & \textcolor{blue}{X}                     & \textcolor{blue}{X}                      & 1                       & \textcolor{blue}{X}                      \\ 
\hline
\textbf{Videology}                                   & \textcolor{blue}{X}                     & 3                       & \textcolor{blue}{X}                     & 1                      & \textcolor{blue}{X}                       & 6                      \\ 
\hline
\textbf{Federated Media}                             & \textcolor{blue}{X}                     & 5                       & \textcolor{blue}{X}                     & \textcolor{blue}{X}                      & 2                       & \textcolor{blue}{X}                      \\ 
\hline
\textbf{ZypMedia}                                    & \textcolor{blue}{X}                     & 4                       & \textcolor{blue}{X}                     & \textcolor{blue}{X}                      & \textcolor{blue}{X}                       & 1                      \\ 
\hline
\textbf{Adotmob}                                     & \textcolor{blue}{X}                     & 3                       & \textcolor{blue}{X}                     & 1                      & \textcolor{blue}{X}                       & \textcolor{blue}{X}                      \\ 
\hline
\textbf{Adventori}                                   & \textcolor{blue}{X}                     & 1                       & \textcolor{blue}{X}                     & \textcolor{blue}{X}                      & \textcolor{blue}{X}                       & \textcolor{blue}{X}                      \\ 
\hline
\textbf{Acuity}                                      & \textcolor{blue}{X}                     & 1                       & \textcolor{blue}{X}                     & 2                      & 1                       & \textcolor{blue}{X}                      \\ 
\hline
\textbf{DynAdmic}                                    & \textcolor{blue}{X}                     & 2                       & \textcolor{blue}{X}                     & 3                      & 1                       & \textcolor{blue}{X}                      \\ 
\hline
\textbf{Lotame}                                      & \textcolor{blue}{X}                     & 1                       & \textcolor{blue}{X}                     & \textcolor{blue}{X}                      & \textcolor{blue}{X}                       & \textcolor{blue}{X}                      \\ 
\hline
\textbf{Amobee}                                      & \textcolor{blue}{X}                     & 2                       & \textcolor{blue}{X}                     & \textcolor{blue}{X}                      & \textcolor{blue}{X}                       & \textcolor{blue}{X}                      \\ 
\hline
\textbf{AdStir}                                      & \textcolor{blue}{X}                     & 1                       & 1                     & \textcolor{blue}{X}                      & \textcolor{blue}{X}                       & \textcolor{blue}{X}                      \\ 
\hline
\textbf{Shareaholic}                                 & \textcolor{blue}{X}                     & 1                       & \textcolor{blue}{X}                     & \textcolor{blue}{X}                      & \textcolor{blue}{X}                       & \textcolor{blue}{X}                      \\ 
\hline
\textbf{Nexage}                                      & \textcolor{blue}{X}                     & \textcolor{blue}{X}                       & 16                    & \textcolor{blue}{X}                      & \textcolor{blue}{X}                       & 16                     \\ 
\hline
\textbf{Specific Media}                              & \textcolor{blue}{X}                     & \textcolor{blue}{X}                       & 16                    & \textcolor{blue}{X}                      & \textcolor{blue}{X}                       & 16                     \\ 
\hline
\textbf{Vibrant Media}                               & \textcolor{blue}{X}                     & \textcolor{blue}{X}                       & 16                    & \textcolor{blue}{X}                      & \textcolor{blue}{X}                       & 16                     \\ 
\hline
\textbf{Cox Digital Solutions}                       & \textcolor{blue}{X}                     & \textcolor{blue}{X}                       & 1                     & \textcolor{blue}{X}                      & \textcolor{blue}{X}                       & \textcolor{blue}{X}                      \\ 
\hline
\textbf{RadiumOne}                                   & \textcolor{blue}{X}                     & \textcolor{blue}{X}                       & 1                     & \textcolor{blue}{X}                      & \textcolor{blue}{X}                       & \textcolor{blue}{X}                      \\ 
\hline
\textbf{RoqAd}                                       & \textcolor{blue}{X}                     & \textcolor{blue}{X}                       & 1                     & 3                      & \textcolor{blue}{X}                       & \textcolor{blue}{X}                      \\ 
\hline
\textbf{Tapad}                                       & \textcolor{blue}{X}                     & \textcolor{blue}{X}                       & \textcolor{blue}{X}                     & 11                     & 11                      & \textcolor{blue}{X}                      \\ 
\hline
\textbf{CONTEXTWEB}                                  & \textcolor{blue}{X}                     & \textcolor{blue}{X}                       & \textcolor{blue}{X}                     & 3                      & 4                       & \textcolor{blue}{X}                      \\ 
\hline
\textbf{BlueKai}                                     & \textcolor{blue}{X}                     & \textcolor{blue}{X}                       & \textcolor{blue}{X}                     & 2                      & 1                       & \textcolor{blue}{X}                      \\ 
\hline
\textbf{Admedo}                                      & \textcolor{blue}{X}                     & \textcolor{blue}{X}                       & \textcolor{blue}{X}                     & 3                      & 1                       & 1                      \\ 
\hline
\textbf{TheReachGroup}                               & \textcolor{blue}{X}                     & \textcolor{blue}{X}                       & \textcolor{blue}{X}                     & 2                      & 3                       & 2                      \\ 
\hline
\textbf{Delta Projects}                              & \textcolor{blue}{X}                     & \textcolor{blue}{X}                       & \textcolor{blue}{X}                     & 2                      & 4                       & 4                      \\ 
\hline
\textbf{SpotXchange}                                 & \textcolor{blue}{X}                     & \textcolor{blue}{X}                       & \textcolor{blue}{X}                     & 1                      & 8                       & \textcolor{blue}{X}                      \\ 
\hline
\textbf{Gemius}                                      & \textcolor{blue}{X}                     & \textcolor{blue}{X}                       & \textcolor{blue}{X}                     & 1                      & \textcolor{blue}{X}                       & 2                      \\ 
\hline
\textbf{Adomik}                                      & \textcolor{blue}{X}                     & \textcolor{blue}{X}                       & \textcolor{blue}{X}                     & 1                      & \textcolor{blue}{X}                       & 1                      \\ 
\hline
\textbf{Deep Intent}                                 & \textcolor{blue}{X}                     & \textcolor{blue}{X}                       & \textcolor{blue}{X}                     & 1                      & \textcolor{blue}{X}                       & \textcolor{blue}{X}                      \\ 
\hline
\textbf{33Across}                                    & \textcolor{blue}{X}                     & \textcolor{blue}{X}                       & \textcolor{blue}{X}                     & \textcolor{blue}{X}                      & 11                      & \textcolor{blue}{X}                      \\ 
\hline
\textbf{Chartbeat}                                   & \textcolor{blue}{X}                     & \textcolor{blue}{X}                       & \textcolor{blue}{X}                     & \textcolor{blue}{X}                      & 11                      & \textcolor{blue}{X}                      \\ 
\hline
\textbf{Nativo}                                      & \textcolor{blue}{X}                     & \textcolor{blue}{X}                       & \textcolor{blue}{X}                     & \textcolor{blue}{X}                      & 10                      & \textcolor{blue}{X}                      \\ 
\hline
\textbf{TripleLift}                                  & \textcolor{blue}{X}                     & \textcolor{blue}{X}                       & \textcolor{blue}{X}                     & \textcolor{blue}{X}                      & 12                      & \textcolor{blue}{X}                      \\ 
\hline
\textbf{Disqus}                                      & \textcolor{blue}{X}                     & \textcolor{blue}{X}                       & \textcolor{blue}{X}                     & \textcolor{blue}{X}                      & 2                       & 2                      \\ 
\hline
\textbf{Conviva}                                     & \textcolor{blue}{X}                     & \textcolor{blue}{X}                       & \textcolor{blue}{X}                     & \textcolor{blue}{X}                      & 2                       & \textcolor{blue}{X}                      \\ 
\hline
\textbf{Kargo}                                       & \textcolor{blue}{X}                     & \textcolor{blue}{X}                       & \textcolor{blue}{X}                     & \textcolor{blue}{X}                      & 3                       & \textcolor{blue}{X}                      \\ 
\hline
\textbf{Sharethrough}                                & \textcolor{blue}{X}                     & \textcolor{blue}{X}                       & \textcolor{blue}{X}                     & \textcolor{blue}{X}                      & 6                       & \textcolor{blue}{X}                      \\ 
\hline
\textbf{INFOnline}                                   & \textcolor{blue}{X}                     & \textcolor{blue}{X}                       & \textcolor{blue}{X}                     & \textcolor{blue}{X}                      & 4                       & \textcolor{blue}{X}                      \\ 
\hline
\textbf{Integral Ad Science}                         & \textcolor{blue}{X}                     & \textcolor{blue}{X}                       & \textcolor{blue}{X}                     & \textcolor{blue}{X}                      & 3                       & \textcolor{blue}{X}                      \\ 
\hline
\textbf{MobFox}                                      & \textcolor{blue}{X}                     & \textcolor{blue}{X}                       & \textcolor{blue}{X}                     & \textcolor{blue}{X}                      & 1                       & \textcolor{blue}{X}                      \\ 
\hline
\textbf{RTBHouse}                                    & \textcolor{blue}{X}                     & \textcolor{blue}{X}                       & \textcolor{blue}{X}                     & \textcolor{blue}{X}                      & 5                       & \textcolor{blue}{X}                      \\ 
\hline
\textbf{OwnerIQ}                                     & \textcolor{blue}{X}                     & \textcolor{blue}{X}                       & \textcolor{blue}{X}                     & \textcolor{blue}{X}                      & 1                       & 8                      \\ 
\hline
\textbf{Taboola}                                     & \textcolor{blue}{X}                     & \textcolor{blue}{X}                       & \textcolor{blue}{X}                     & \textcolor{blue}{X}                      & 3                       & \textcolor{blue}{X}                      \\ 
\hline
\textbf{Rhythm}                                      & \textcolor{blue}{X}                     & \textcolor{blue}{X}                       & \textcolor{blue}{X}                     & \textcolor{blue}{X}                      & 2                       & \textcolor{blue}{X}                      \\ 
\hline
\textbf{OpenX}                                       & \textcolor{blue}{X}                     & \textcolor{blue}{X}                       & \textcolor{blue}{X}                     & \textcolor{blue}{X}                      & 3                       & \textcolor{blue}{X}                      \\ 
\hline
\textbf{AK}                                          & \textcolor{blue}{X}                     & \textcolor{blue}{X}                       & \textcolor{blue}{X}                     & \textcolor{blue}{X}                      & 1                       & 2                      \\ 
\hline
\textbf{Rocket Fuel}                                 & \textcolor{blue}{X}                     & \textcolor{blue}{X}                       & \textcolor{blue}{X}                     & \textcolor{blue}{X}                      & 1                       & \textcolor{blue}{X}                      \\
\hline
\end{tabular}
\end{table*}

\subsection{\textcolor{blue}{Do advertisers \& trackers obey Opt-out?}}

\textcolor{blue}{In this section, we will discuss if any advertisers, bidders or other third party service obey or disobey the opt-out, based on the HTTP data and bids data.}

\subsubsection{\textcolor{blue}{Who apppeared before opt-out and disappeared after opt-out?}}

\textcolor{blue}{Table \ref{tbl:in_train_not_in_test_1} to Table \ref{tbl:in_train_not_in_test_5} represented the summary of advertisers, bidders or other third party service who disappeared after opt-out. The first column is the name of advertisers, bidders, or other third party service names. The number in specific column represents the number of personas (total number of personas is 16). }

\textcolor{blue}{For example, in Table \ref{tbl:in_train_not_in_test_1}, advertiser \textbf{IAB} has number \textbf{1} in Setting \textbf{Onetrust CA}. This represent \textbf{IAB} disappeared in 1 persona in the setting CMP: \textbf{Onetrust} with \textbf{California IPs} after opt-out. Blue \textbf{X} represents this advertiser, bidder, or other third party service did not meet the analysis condition: "appeared before opt-out and disappeared after opt-out" in the current CMP-IP setting. We also do not consider the advertiser, bidder, or other third party service who appeared in both before and after opt-out.}

\textcolor{blue}{Conclusion: Some Advertisers/Bidders/3rd Party service do obey the opt-out, like \textbf{Markit} in the setting \textbf{Central CA} having all 16 personas opt-out in Table \ref{tbl:in_train_not_in_test_1}}

\subsubsection{\textcolor{blue}{Who did not exist before opt-out but appeared after opt-out?}}

\begin{table*}
\centering
	\caption{The summary of bidders that did not appear before opt-out and appeared after opt-out in bids data}
	\label{tbl:in_test_not_in_train}
\begin{tabular}{|l|l|l|l|l|l|l|} 
\hline
\textbf{Bidders}                           & \textbf{Onetrust\_CA} & \textbf{~Cookiebot\_CA} & \textbf{~Central\_CA} & \textbf{~Onetrust\_GE} & \textbf{~Cookiebot\_GE} & \textbf{~Central\_GE}  \\ 
\hline
\textbf{SmartAdServer}                     & X                     & X                       & 8                     & X                      & X                       & X                      \\ 
\hline
\textbf{Teads.tv} & X                     & X                       & X                     & X                      & X                       & 1                      \\
\hline
\end{tabular}
\end{table*}

\begin{table*}
\centering
	\caption{The summary of bidders that did not appear before opt-out and appeared after opt-out in HTTP data, part 1}
	\label{tbl:in_test_not_in_train_1}
\begin{tabular}{|l|l|l|l|l|l|l|} 
\hline
\textbf{Advertiser/Bidders/3rd Party Service}    & \textbf{Onetrust\_CA} & \textbf{~Cookiebot\_CA} & \textbf{~Central\_CA} & \textbf{~Onetrust\_GE} & \textbf{~Cookiebot\_GE} & \textbf{~Central\_GE}  \\ 
\hline
\textbf{FreeWheel}                               & 1                     & 2                       & \textcolor{blue}{X}                    & 4                      & 4                       & 2                      \\ 
\hline
\textbf{Survata}                                 & 1                     & \textcolor{blue}{X}                      & 2                     & 6                      & \textcolor{blue}{X}                      & \textcolor{blue}{X}                     \\ 
\hline
\textbf{DG}                                      & 1                     & 1                       & 4                     & 3                      & \textcolor{blue}{X}                      & \textcolor{blue}{X}                     \\ 
\hline
\textbf{Semasio}                                 & 2                     & 2                       & \textcolor{blue}{X}                    & 4                      & 8                       & \textcolor{blue}{X}                     \\ 
\hline
\textbf{Conviva}                                 & 14                    & \textcolor{blue}{X}                      & 14                    & 11                     & \textcolor{blue}{X}                      & 14                     \\ 
\hline
\textbf{Lotame}                                  & 1                     & 1                       & \textcolor{blue}{X}                    & 1                      & 3                       & \textcolor{blue}{X}                     \\ 
\hline
\textbf{EQ Ads}                                  & 4                     & 6                       & 3                     & 8                      & 8                       & 7                      \\ 
\hline
\textbf{AdvancedStore}                           & 6                     & 6                       & 1                     & 10                     & 13                      & 9                      \\ 
\hline
\textbf{Bidtellect}                              & 1                     & 1                       & 1                     & 8                      & 13                      & 13                     \\ 
\hline
\textbf{ucfunnel}                                & 9                     & \textcolor{blue}{X}                      & 13                    & \textcolor{blue}{X}                     & \textcolor{blue}{X}                      & 16                     \\ 
\hline
\textbf{ZypMedia}                                & 2                     & 5                       & 4                     & 13                     & 11                      & 7                      \\ 
\hline
\textbf{BidTheatre}                              & 6                     & 7                       & 7                     & 10                     & 11                      & 10                     \\ 
\hline
\textbf{Akamai}                                  & 1                     & \textcolor{blue}{X}                      & 1                     & 1                      & \textcolor{blue}{X}                      & 1                      \\ 
\hline
\textbf{Nielsen}                                 & 4                     & 2                       & 5                     & 9                      & \textcolor{blue}{X}                      & 9                      \\ 
\hline
\textbf{Kargo}                                   & 5                     & 6                       & \textcolor{blue}{X}                    & 13                     & \textcolor{blue}{X}                      & \textcolor{blue}{X}                     \\ 
\hline
\textbf{4INFO}                                   & 7                     & 5                       & \textcolor{blue}{X}                    & \textcolor{blue}{X}                     & \textcolor{blue}{X}                      & \textcolor{blue}{X}                     \\ 
\hline
\textbf{JustPremium}                             & 8                     & 6                       & 7                     & 10                     & \textcolor{blue}{X}                      & 9                      \\ 
\hline
\textbf{IponWeb}                                 & 3                     & 1                       & 10                    & \textcolor{blue}{X}                     & \textcolor{blue}{X}                      & \textcolor{blue}{X}                     \\ 
\hline
\textbf{Videology}                               & 6                     & 4                       & \textcolor{blue}{X}                    & 5                      & 7                       & 3                      \\ 
\hline
\textbf{Brightcove}                              & 7                     & \textcolor{blue}{X}                      & 7                     & 5                      & \textcolor{blue}{X}                      & 6                      \\ 
\hline
\textbf{Tealium}                                 & 6                     & \textcolor{blue}{X}                      & \textcolor{blue}{X}                    & 9                      & \textcolor{blue}{X}                      & \textcolor{blue}{X}                     \\ 
\hline
\textbf{Bombora}                                 & 3                     & \textcolor{blue}{X}                      & 5                     & 1                      & \textcolor{blue}{X}                      & \textcolor{blue}{X}                     \\ 
\hline
\textbf{Drawbridge}                              & 1                     & 1                       & 1                     & \textcolor{blue}{X}                     & \textcolor{blue}{X}                      & 16                     \\ 
\hline
\textbf{ShareThis}                               & 7                     & \textcolor{blue}{X}                      & \textcolor{blue}{X}                    & \textcolor{blue}{X}                     & \textcolor{blue}{X}                      & \textcolor{blue}{X}                     \\ 
\hline
\textbf{iBehavior}                               & 2                     & \textcolor{blue}{X}                      & \textcolor{blue}{X}                    & \textcolor{blue}{X}                     & \textcolor{blue}{X}                      & \textcolor{blue}{X}                     \\ 
\hline
\textbf{cXense}                                  & 10                    & \textcolor{blue}{X}                      & \textcolor{blue}{X}                    & 10                     & \textcolor{blue}{X}                      & \textcolor{blue}{X}                     \\ 
\hline
\textbf{TubeMogul}                               & 9                     & \textcolor{blue}{X}                      & 9                     & \textcolor{blue}{X}                     & 1                       & 1                      \\ 
\hline
\textbf{Storygize}                               & 3                     & 3                       & 9                     & 1                      & \textcolor{blue}{X}                      & 15                     \\ 
\hline
\textbf{ADITION}                                 & 7                     & 6                       & 7                     & 7                      & 10                      & 6                      \\ 
\hline
\textbf{AdYouLike}                               & 5                     & 5                       & 8                     & \textcolor{blue}{X}                     & 3                       & 13                     \\ 
\hline
\textbf{AvidMedia}                               & 9                     & 2                       & 15                    & \textcolor{blue}{X}                     & \textcolor{blue}{X}                      & 16                     \\ 
\hline
\textbf{Disqus}                                  & 16                    & 16                      & \textcolor{blue}{X}                    & 14                     & \textcolor{blue}{X}                      & \textcolor{blue}{X}                     \\ 
\hline
\textbf{Betgenius}                               & 2                     & 3                       & 5                     & \textcolor{blue}{X}                     & \textcolor{blue}{X}                      & \textcolor{blue}{X}                     \\ 
\hline
\textbf{LiveRamp}                                & 3                     & 1                       & 5                     & \textcolor{blue}{X}                     & \textcolor{blue}{X}                      & 11                     \\ 
\hline
\textbf{DoubleVerify}                            & 1                     & \textcolor{blue}{X}                      & 2                     & 2                      & 3                       & 7                      \\ 
\hline
\textbf{Parse.ly}    & 4                     & \textcolor{blue}{X}                      & 6                     & 8                      & 8                       & \textcolor{blue}{X}                     \\ 
\hline
\textbf{SpringServe}                             & 7                     & \textcolor{blue}{X}                      & 15                    & 15                     & \textcolor{blue}{X}                      & 15                     \\ 
\hline
\textbf{LKQD}                                    & 4                     & 1                       & 7                     & \textcolor{blue}{X}                     & \textcolor{blue}{X}                      & 5                      \\ 
\hline
\textbf{Proclivity}                              & 3                     & 3                       & 4                     & \textcolor{blue}{X}                     & \textcolor{blue}{X}                      & \textcolor{blue}{X}                     \\ 
\hline
\textbf{Sojern}                                  & 2                     & 1                       & 6                     & \textcolor{blue}{X}                     & \textcolor{blue}{X}                      & \textcolor{blue}{X}                     \\ 
\hline
\textbf{RichAudience}                            & 7                     & \textcolor{blue}{X}                      & 11                    & 15                     & \textcolor{blue}{X}                      & 14                     \\ 
\hline
\textbf{AddThis}                                 & 1                     & 2                       & \textcolor{blue}{X}                    & 4                      & 4                       & \textcolor{blue}{X}                     \\ 
\hline
\textbf{ClickDistrict}                           & 3                     & 2                       & 3                     & 2                      & 8                       & 16                     \\ 
\hline
\textbf{Research Now}                            & 2                     & \textcolor{blue}{X}                      & 5                     & \textcolor{blue}{X}                     & \textcolor{blue}{X}                      & \textcolor{blue}{X}                     \\ 
\hline
\textbf{Fluct}                                   & 5                     & 2                       & 7                     & \textcolor{blue}{X}                     & \textcolor{blue}{X}                      & \textcolor{blue}{X}                     \\ 
\hline
\textbf{Jivox}                                   & 2                     & \textcolor{blue}{X}                      & 4                     & \textcolor{blue}{X}                     & \textcolor{blue}{X}                      & \textcolor{blue}{X}                     \\ 
\hline
\textbf{ADP Dealer Services}                     & 1                     & \textcolor{blue}{X}                      & 1                     & \textcolor{blue}{X}                     & \textcolor{blue}{X}                      & \textcolor{blue}{X}                     \\ 
\hline
\textbf{BrightTag}                               & 3                     & 1                       & 13                    & \textcolor{blue}{X}                     & 13                      & 13                     \\ 
\hline
\textbf{ID5}                                     & 2                     & 1                       & 3                     & 3                      & 6                       & 5                      \\ 
\hline
\textbf{Flashtalking}                            & 2                     & 3                       & \textcolor{blue}{X}                    & 1                      & \textcolor{blue}{X}                      & \textcolor{blue}{X}                     \\ 
\hline
\textbf{C3 Metrics}                              & 1                     & \textcolor{blue}{X}                      & 8                     & \textcolor{blue}{X}                     & \textcolor{blue}{X}                      & \textcolor{blue}{X}                     \\ 
\hline
\textbf{MobileAdTrading}                         & 1                     & \textcolor{blue}{X}                      & 12                    & \textcolor{blue}{X}                     & \textcolor{blue}{X}                      & \textcolor{blue}{X}                     \\ 
\hline
\textbf{FreakOut}                                & 1                     & \textcolor{blue}{X}                      & 11                    & \textcolor{blue}{X}                     & \textcolor{blue}{X}                      & \textcolor{blue}{X}                     \\ 
\hline
\textbf{Tremor Video}                            & 3                     & 4                       & \textcolor{blue}{X}                    & 4                      & \textcolor{blue}{X}                      & \textcolor{blue}{X}                     \\ 
\hline
\textbf{AdRoll}                                  & 2                     & 3                       & \textcolor{blue}{X}                    & 10                     & 10                      & \textcolor{blue}{X}                     \\ 
\hline
\textbf{Chartbeat}                               & 2                     & 2                       & 2                     & 4                      & \textcolor{blue}{X}                      & 4                      \\ 
\hline
\textbf{Choozle}                                 & 1                     & 1                       & \textcolor{blue}{X}                    & \textcolor{blue}{X}                     & \textcolor{blue}{X}                      & \textcolor{blue}{X}                     \\ 
\hline
\textbf{Technorati}                              & 2                     & 2                       & 2                     & 11                     & \textcolor{blue}{X}                      & 13                     \\ 
\hline
\textbf{Outbrain}                                & 1                     & 1                       & \textcolor{blue}{X}                    & \textcolor{blue}{X}                     & 7                       & \textcolor{blue}{X}                     \\ 
\hline
\textbf{Salesforce.com} & 2                     & \textcolor{blue}{X}                      & 2                     & 3                      & \textcolor{blue}{X}                      & 3                      \\ 
\hline
\textbf{Narrative}                               & 2                     & 4                       & 2                     & \textcolor{blue}{X}                     & \textcolor{blue}{X}                      & \textcolor{blue}{X}                     \\ 
\hline
\textbf{Adotmob}                                 & 2                     & 5                       & 5                     & 10                     & 13                      & 9                      \\ 
\hline
\textbf{Moat}                                    & 1                     & 1                       & 2                     & 1                      & 1                       & 1                      \\ 
\hline
\textbf{WPP}                                     & 1                     & 2                       & \textcolor{blue}{X}                    & 3                      & 4                       & \textcolor{blue}{X}                     \\ 
\hline
\textbf{Adform}                                  & 1                     & 1                       & \textcolor{blue}{X}                    & 2                      & 4                       & \textcolor{blue}{X}                     \\ 
\hline
\textbf{33Across}                                & 1                     & 1                       & \textcolor{blue}{X}                    & 4                      & \textcolor{blue}{X}                      & \textcolor{blue}{X}                     \\ 
\hline
\textbf{DynAdmic}                                & 1                     & 2                       & 2                     & 11                     & 7                       & 12                     \\ 
\hline
\end{tabular}
\end{table*}

\begin{table*}
\centering
	\caption{The summary of bidders that did not appear before opt-out and appeared after opt-out in HTTP data, part 2}
	\label{tbl:in_test_not_in_train_2}
\begin{tabular}{|l|l|l|l|l|l|l|}

\hline
\textbf{Advertiser/Bidders/3rd Party Service}                           & \textbf{Onetrust\_CA} & \textbf{~Cookiebot\_CA} & \textbf{~Central\_CA} & \textbf{~Onetrust\_GE} & \textbf{~Cookiebot\_GE} & \textbf{~Central\_GE}  \\ 
\hline
\textbf{Sharethrough}                            & 1                     & \textcolor{blue}{X}                      & \textcolor{blue}{X}                    & 7                      & 2                       & 6                      \\ 
\hline
\textbf{Yieldmo}                                 & 1                     & 1                       & \textcolor{blue}{X}                    & \textcolor{blue}{X}                     & 14                      & \textcolor{blue}{X}                     \\ 
\hline
\textbf{CONTEXTWEB}                              & 1                     & 1                       & \textcolor{blue}{X}                    & 6                      & 3                       & 11                     \\ 
\hline
\textbf{DistrictM}                               & 1                     & 2                       & 1                     & 15                     & \textcolor{blue}{X}                      & 15                     \\ 
\hline
\textbf{Bidr}                                    & 1                     & 2                       & \textcolor{blue}{X}                    & 6                      & 5                       & \textcolor{blue}{X}                     \\ 
\hline
\textbf{engage:BDR}                              & 2                     & 3                       & 3                     & 11                     & 7                       & 14                     \\ 
\hline
\textbf{OnAudience}                              & 1                     & 4                       & 2                     & 5                      & 5                       & 4                      \\ 
\hline
\textbf{AdGear}                                  & 1                     & 2                       & 3                     & 10                     & 12                      & 11                     \\ 
\hline
\textbf{MaxPoint}                                & 1                     & \textcolor{blue}{X}                      & 2                     & 15                     & 10                      & 8                      \\ 
\hline
\textbf{Deep Intent}                             & 1                     & 1                       & 1                     & 8                      & 9                       & 9                      \\ 
\hline
\textbf{GumGum}                                  & 1                     & 1                       & \textcolor{blue}{X}                    & 8                      & 6                       & \textcolor{blue}{X}                     \\ 
\hline
\textbf{Appier}                                  & 2                     & 4                       & 2                     & 6                      & 6                       & 16                     \\ 
\hline
\textbf{Rocket Fuel}                             & 1                     & 1                       & 1                     & 5                      & 6                       & 7                      \\ 
\hline
\textbf{Zemanta}                                 & 1                     & 1                       & 1                     & 7                      & 9                       & 11                     \\ 
\hline
\textbf{AdKernel}                                & 1                     & 4                       & 4                     & \textcolor{blue}{X}                     & \textcolor{blue}{X}                      & \textcolor{blue}{X}                     \\ 
\hline
\textbf{Adscience}                               & 1                     & \textcolor{blue}{X}                      & 2                     & \textcolor{blue}{X}                     & \textcolor{blue}{X}                      & \textcolor{blue}{X}                     \\ 
\hline
\textbf{BoostBox}                                & \textcolor{blue}{X}                    & 3                       & \textcolor{blue}{X}                    & \textcolor{blue}{X}                     & \textcolor{blue}{X}                      & \textcolor{blue}{X}                     \\ 
\hline
\textbf{Simpli.fi}     & \textcolor{blue}{X}                    & 1                       & \textcolor{blue}{X}                    & 4                      & 5                       & \textcolor{blue}{X}                     \\ 
\hline
\textbf{SiteScout}                               & \textcolor{blue}{X}                    & 1                       & \textcolor{blue}{X}                    & 2                      & 4                       & 2                      \\ 
\hline
\textbf{Tapad}                                   & \textcolor{blue}{X}                    & 1                       & \textcolor{blue}{X}                    & \textcolor{blue}{X}                     & \textcolor{blue}{X}                      & \textcolor{blue}{X}                     \\ 
\hline
\textbf{OwnerIQ}                                 & \textcolor{blue}{X}                    & 1                       & \textcolor{blue}{X}                    & 12                     & 12                      & \textcolor{blue}{X}                     \\ 
\hline
\textbf{media.net}      & \textcolor{blue}{X}                    & 1                       & \textcolor{blue}{X}                    & 4                      & 3                       & \textcolor{blue}{X}                     \\ 
\hline
\textbf{Admeta}                                  & \textcolor{blue}{X}                    & 15                      & 11                    & \textcolor{blue}{X}                     & \textcolor{blue}{X}                      & \textcolor{blue}{X}                     \\ 
\hline
\textbf{Adswizz}                                 & \textcolor{blue}{X}                    & 11                      & 9                     & \textcolor{blue}{X}                     & \textcolor{blue}{X}                      & \textcolor{blue}{X}                     \\ 
\hline
\textbf{Acuity}                                  & \textcolor{blue}{X}                    & 1                       & \textcolor{blue}{X}                    & 5                      & 6                       & \textcolor{blue}{X}                     \\ 
\hline
\textbf{DataXu}                                  & \textcolor{blue}{X}                    & 1                       & \textcolor{blue}{X}                    & 4                      & 3                       & 3                      \\ 
\hline
\textbf{AK}                                      & \textcolor{blue}{X}                    & 1                       & \textcolor{blue}{X}                    & 1                      & 3                       & \textcolor{blue}{X}                     \\ 
\hline
\textbf{TRUSTe}                                  & \textcolor{blue}{X}                    & 1                       & 2                     & 1                      & 1                       & 3                      \\ 
\hline
\textbf{eXelate}                                 & \textcolor{blue}{X}                    & 1                       & \textcolor{blue}{X}                    & 2                      & 4                       & \textcolor{blue}{X}                     \\ 
\hline
\textbf{Caraytech}                               & \textcolor{blue}{X}                    & 1                       & 11                    & \textcolor{blue}{X}                     & \textcolor{blue}{X}                      & \textcolor{blue}{X}                     \\ 
\hline
\textbf{Krux}                                    & \textcolor{blue}{X}                    & 1                       & \textcolor{blue}{X}                    & 1                      & 2                       & \textcolor{blue}{X}                     \\ 
\hline
\textbf{Acxiom}                                  & \textcolor{blue}{X}                    & 1                       & \textcolor{blue}{X}                    & \textcolor{blue}{X}                     & \textcolor{blue}{X}                      & \textcolor{blue}{X}                     \\ 
\hline
\textbf{BlueKai}                                 & \textcolor{blue}{X}                    & 1                       & \textcolor{blue}{X}                    & 1                      & 2                       & \textcolor{blue}{X}                     \\ 
\hline
\textbf{Resonate}                                & \textcolor{blue}{X}                    & 3                       & 5                     & \textcolor{blue}{X}                     & \textcolor{blue}{X}                      & \textcolor{blue}{X}                     \\ 
\hline
\textbf{Bouncex}                                 & \textcolor{blue}{X}                    & 2                       & 2                     & 5                      & \textcolor{blue}{X}                      & 5                      \\ 
\hline
\textbf{Merkle}                                  & \textcolor{blue}{X}                    & 2                       & 3                     & 7                      & 7                       & 7                      \\ 
\hline
\textbf{eBay}                                    & \textcolor{blue}{X}                    & 3                       & 4                     & 2                      & \textcolor{blue}{X}                      & 3                      \\ 
\hline
\textbf{Sonobi}                                  & \textcolor{blue}{X}                    & 2                       & \textcolor{blue}{X}                    & 3                      & 6                       & \textcolor{blue}{X}                     \\ 
\hline
\textbf{Federated Media}                         & \textcolor{blue}{X}                    & 1                       & 1                     & 1                      & 2                       & 1                      \\ 
\hline
\textbf{Undertone}                               & \textcolor{blue}{X}                    & 5                       & \textcolor{blue}{X}                    & \textcolor{blue}{X}                     & \textcolor{blue}{X}                      & \textcolor{blue}{X}                     \\ 
\hline
\textbf{SmartAdServer}                           & \textcolor{blue}{X}                    & 1                       & 10                    & \textcolor{blue}{X}                     & \textcolor{blue}{X}                      & 14                     \\ 
\hline
\textbf{Demandbase}                              & \textcolor{blue}{X}                    & 2                       & \textcolor{blue}{X}                    & \textcolor{blue}{X}                     & \textcolor{blue}{X}                      & \textcolor{blue}{X}                     \\ 
\hline
\textbf{Unruly}                                  & \textcolor{blue}{X}                    & 2                       & 3                     & 6                      & 2                       & 7                      \\ 
\hline
\textbf{IAB}                                     & \textcolor{blue}{X}                    & 1                       & 15                    & \textcolor{blue}{X}                     & \textcolor{blue}{X}                      & 16                     \\ 
\hline
\textbf{Quantcast}                               & \textcolor{blue}{X}                    & 1                       & \textcolor{blue}{X}                    & \textcolor{blue}{X}                     & \textcolor{blue}{X}                      & \textcolor{blue}{X}                     \\ 
\hline
\textbf{Integral Ad Science}                     & \textcolor{blue}{X}                    & 1                       & 1                     & 3                      & 2                       & 3                      \\ 
\hline
\textbf{EMX}                                     & \textcolor{blue}{X}                    & 1                       & \textcolor{blue}{X}                    & 7                      & 4                       & \textcolor{blue}{X}                     \\ 
\hline
\textbf{adscale}                                 & \textcolor{blue}{X}                    & \textcolor{blue}{X}                      & 14                    & \textcolor{blue}{X}                     & \textcolor{blue}{X}                      & 13                     \\ 
\hline
\textbf{LinkedIn}                                & \textcolor{blue}{X}                    & \textcolor{blue}{X}                      & 1                     & 1                      & \textcolor{blue}{X}                      & 2                      \\ 
\hline
\textbf{TrustX}                                  & \textcolor{blue}{X}                    & \textcolor{blue}{X}                      & 5                     & 7                      & 8                       & 9                      \\ 
\hline
\textbf{BetweenDigital}                          & \textcolor{blue}{X}                    & \textcolor{blue}{X}                      & 9                     & 14                     & 2                       & 13                     \\ 
\hline
\textbf{GetIntent}                               & \textcolor{blue}{X}                    & \textcolor{blue}{X}                      & 12                    & 1                      & 1                       & 15                     \\ 
\hline
\textbf{MTS}                                     & \textcolor{blue}{X}                    & \textcolor{blue}{X}                      & 7                     & \textcolor{blue}{X}                     & \textcolor{blue}{X}                      & 2                      \\ 
\hline
\textbf{RuTarget}                                & \textcolor{blue}{X}                    & \textcolor{blue}{X}                      & 5                     & \textcolor{blue}{X}                     & \textcolor{blue}{X}                      & \textcolor{blue}{X}                     \\ 
\hline
\textbf{AdRiver}                                 & \textcolor{blue}{X}                    & \textcolor{blue}{X}                      & 14                    & \textcolor{blue}{X}                     & \textcolor{blue}{X}                      & 15                     \\ 
\hline
\textbf{Optimizely}                              & \textcolor{blue}{X}                    & \textcolor{blue}{X}                      & 1                     & \textcolor{blue}{X}                     & \textcolor{blue}{X}                      & \textcolor{blue}{X}                     \\ 
\hline
\textbf{Sourcepoint}                             & \textcolor{blue}{X}                    & \textcolor{blue}{X}                      & 11                    & 13                     & \textcolor{blue}{X}                      & \textcolor{blue}{X}                     \\ 
\hline
\textbf{IntimateMerger}                          & \textcolor{blue}{X}                    & \textcolor{blue}{X}                      & 10                    & \textcolor{blue}{X}                     & \textcolor{blue}{X}                      & 1                      \\ 
\hline
\textbf{Powerlinks}                              & \textcolor{blue}{X}                    & \textcolor{blue}{X}                      & 10                    & \textcolor{blue}{X}                     & \textcolor{blue}{X}                      & \textcolor{blue}{X}                     \\ 
\hline
\textbf{Datalogix}                               & \textcolor{blue}{X}                    & \textcolor{blue}{X}                      & 12                    & \textcolor{blue}{X}                     & \textcolor{blue}{X}                      & \textcolor{blue}{X}                     \\ 
\hline
\textbf{Innity}                                  & \textcolor{blue}{X}                    & \textcolor{blue}{X}                      & 16                    & \textcolor{blue}{X}                     & \textcolor{blue}{X}                      & 16                     \\ 
\hline
\textbf{TheTimesGroup}                           & \textcolor{blue}{X}                    & \textcolor{blue}{X}                      & 12                    & \textcolor{blue}{X}                     & \textcolor{blue}{X}                      & 12                     \\ 
\hline
\textbf{LiveInternet}                            & \textcolor{blue}{X}                    & \textcolor{blue}{X}                      & 15                    & \textcolor{blue}{X}                     & \textcolor{blue}{X}                      & 15                     \\ 
\hline
\textbf{Mail.Ru}                                 & \textcolor{blue}{X}                    & \textcolor{blue}{X}                      & 16                    & 16                     & \textcolor{blue}{X}                      & 16                     \\ 
\hline
\textbf{AdFox}                                   & \textcolor{blue}{X}                    & \textcolor{blue}{X}                      & 14                    & \textcolor{blue}{X}                     & \textcolor{blue}{X}                      & 14                     \\ 
\hline
\textbf{Connatix.com}  & \textcolor{blue}{X}                    & \textcolor{blue}{X}                      & 11                    & 5                      & \textcolor{blue}{X}                      & 12                     \\ 
\hline
\textbf{InsightExpress}                          & \textcolor{blue}{X}                    & \textcolor{blue}{X}                      & 7                     & \textcolor{blue}{X}                     & \textcolor{blue}{X}                      & 1                      \\ 
\hline
\end{tabular}
\end{table*}

\begin{table*}
\centering
	\caption{The summary of bidders that did not appear before opt-out and appeared after opt-out in HTTP data, part 3}
	\label{tbl:in_test_not_in_train_3}
\begin{tabular}{|l|l|l|l|l|l|l|} 
\hline
\textbf{Advertiser/Bidders/3rd Party Service}                           & \textbf{Onetrust\_CA} & \textbf{~Cookiebot\_CA} & \textbf{~Central\_CA} & \textbf{~Onetrust\_GE} & \textbf{~Cookiebot\_GE} & \textbf{~Central\_GE}  \\ 
\hline

\textbf{InMobi}                                  & \textcolor{blue}{X}                    & \textcolor{blue}{X}                      & 4                     & \textcolor{blue}{X}                     & \textcolor{blue}{X}                      & \textcolor{blue}{X}                     \\ 
\hline
\textbf{m6d}                                     & \textcolor{blue}{X}                    & \textcolor{blue}{X}                      & 1                     & \textcolor{blue}{X}                     & \textcolor{blue}{X}                      & \textcolor{blue}{X}                     \\ 
\hline
\textbf{Cox Digital Solutions}                   & \textcolor{blue}{X}                    & \textcolor{blue}{X}                      & 1                     & \textcolor{blue}{X}                     & \textcolor{blue}{X}                      & \textcolor{blue}{X}                     \\ 
\hline
\textbf{SnowplowAnalytics}                       & \textcolor{blue}{X}                    & \textcolor{blue}{X}                      & 11                    & \textcolor{blue}{X}                     & \textcolor{blue}{X}                      & \textcolor{blue}{X}                     \\ 
\hline
\textbf{AT Internet}                             & \textcolor{blue}{X}                    & \textcolor{blue}{X}                      & 15                    & \textcolor{blue}{X}                     & \textcolor{blue}{X}                      & 15                     \\ 
\hline
\textbf{Keywee}                                  & \textcolor{blue}{X}                    & \textcolor{blue}{X}                      & 12                    & \textcolor{blue}{X}                     & \textcolor{blue}{X}                      & \textcolor{blue}{X}                     \\ 
\hline
\textbf{LockerDome}                              & \textcolor{blue}{X}                    & \textcolor{blue}{X}                      & 13                    & \textcolor{blue}{X}                     & \textcolor{blue}{X}                      & 15                     \\ 
\hline
\textbf{MailChimp}                               & \textcolor{blue}{X}                    & \textcolor{blue}{X}                      & 14                    & 14                     & \textcolor{blue}{X}                      & 14                     \\ 
\hline
\textbf{RevContent}                              & \textcolor{blue}{X}                    & \textcolor{blue}{X}                      & 13                    & \textcolor{blue}{X}                     & \textcolor{blue}{X}                      & 14                     \\ 
\hline
\textbf{reddit}                                  & \textcolor{blue}{X}                    & \textcolor{blue}{X}                      & 5                     & \textcolor{blue}{X}                     & \textcolor{blue}{X}                      & 8                      \\ 
\hline
\textbf{DigitalAdConsortium}                     & \textcolor{blue}{X}                    & \textcolor{blue}{X}                      & 14                    & \textcolor{blue}{X}                     & \textcolor{blue}{X}                      & 15                     \\ 
\hline
\textbf{MicroAd}                                 & \textcolor{blue}{X}                    & \textcolor{blue}{X}                      & 15                    & \textcolor{blue}{X}                     & \textcolor{blue}{X}                      & 16                     \\ 
\hline
\textbf{Selectable Media}                        & \textcolor{blue}{X}                    & \textcolor{blue}{X}                      & 14                    & 14                     & 14                      & 14                     \\ 
\hline
\textbf{Segment.io} & \textcolor{blue}{X}                    & \textcolor{blue}{X}                      & 9                     & 10                     & \textcolor{blue}{X}                      & 9                      \\ 
\hline
\textbf{AuditedMedia}                            & \textcolor{blue}{X}                    & \textcolor{blue}{X}                      & 14                    & 14                     & \textcolor{blue}{X}                      & 14                     \\ 
\hline
\textbf{Skimlinks}                               & \textcolor{blue}{X}                    & \textcolor{blue}{X}                      & 8                     & 9                      & 9                       & \textcolor{blue}{X}                     \\ 
\hline
\textbf{StatCounter}                             & \textcolor{blue}{X}                    & \textcolor{blue}{X}                      & 16                    & \textcolor{blue}{X}                     & \textcolor{blue}{X}                      & 16                     \\ 
\hline
\textbf{Adiant}                                  & \textcolor{blue}{X}                    & \textcolor{blue}{X}                      & 12                    & \textcolor{blue}{X}                     & \textcolor{blue}{X}                      & \textcolor{blue}{X}                     \\ 
\hline
\textbf{Grapeshot}                               & \textcolor{blue}{X}                    & \textcolor{blue}{X}                      & 15                    & \textcolor{blue}{X}                     & \textcolor{blue}{X}                      & \textcolor{blue}{X}                     \\ 
\hline
\textbf{Gigya}                                   & \textcolor{blue}{X}                    & \textcolor{blue}{X}                      & 9                     & \textcolor{blue}{X}                     & \textcolor{blue}{X}                      & \textcolor{blue}{X}                     \\ 
\hline
\textbf{Branch}                                  & \textcolor{blue}{X}                    & \textcolor{blue}{X}                      & 7                     & \textcolor{blue}{X}                     & \textcolor{blue}{X}                      & \textcolor{blue}{X}                     \\ 
\hline
\textbf{Web.com}     & \textcolor{blue}{X}                    & \textcolor{blue}{X}                      & 15                    & \textcolor{blue}{X}                     & \textcolor{blue}{X}                      & 15                     \\ 
\hline
\textbf{BuySellAds}                              & \textcolor{blue}{X}                    & \textcolor{blue}{X}                      & 14                    & \textcolor{blue}{X}                     & \textcolor{blue}{X}                      & 14                     \\ 
\hline
\textbf{Trafmag}                                 & \textcolor{blue}{X}                    & \textcolor{blue}{X}                      & 13                    & \textcolor{blue}{X}                     & \textcolor{blue}{X}                      & 16                     \\ 
\hline
\textbf{User Local}                              & \textcolor{blue}{X}                    & \textcolor{blue}{X}                      & 15                    & \textcolor{blue}{X}                     & \textcolor{blue}{X}                      & 15                     \\ 
\hline
\textbf{1plusx}                                  & \textcolor{blue}{X}                    & \textcolor{blue}{X}                      & 14                    & \textcolor{blue}{X}                     & \textcolor{blue}{X}                      & 15                     \\ 
\hline
\textbf{Ensighten}                               & \textcolor{blue}{X}                    & \textcolor{blue}{X}                      & 7                     & \textcolor{blue}{X}                     & \textcolor{blue}{X}                      & 7                      \\ 
\hline
\textbf{Mouseflow}                               & \textcolor{blue}{X}                    & \textcolor{blue}{X}                      & 9                     & \textcolor{blue}{X}                     & \textcolor{blue}{X}                      & 13                     \\ 
\hline
\textbf{SiftScience}                             & \textcolor{blue}{X}                    & \textcolor{blue}{X}                      & 12                    & \textcolor{blue}{X}                     & \textcolor{blue}{X}                      & 13                     \\ 
\hline
\textbf{aidata}                                  & \textcolor{blue}{X}                    & \textcolor{blue}{X}                      & 6                     & \textcolor{blue}{X}                     & \textcolor{blue}{X}                      & 12                     \\ 
\hline
\textbf{Crazy Egg}                               & \textcolor{blue}{X}                    & \textcolor{blue}{X}                      & 2                     & 5                      & 5                       & 5                      \\ 
\hline
\textbf{Automattic}                              & \textcolor{blue}{X}                    & \textcolor{blue}{X}                      & 3                     & \textcolor{blue}{X}                     & \textcolor{blue}{X}                      & \textcolor{blue}{X}                     \\ 
\hline
\textbf{TNS}                                     & \textcolor{blue}{X}                    & \textcolor{blue}{X}                      & 3                     & \textcolor{blue}{X}                     & \textcolor{blue}{X}                      & 9                      \\ 
\hline
\textbf{Opera}                                   & \textcolor{blue}{X}                    & \textcolor{blue}{X}                      & 8                     & \textcolor{blue}{X}                     & \textcolor{blue}{X}                      & 13                     \\ 
\hline
\textbf{Adloox}                                  & \textcolor{blue}{X}                    & \textcolor{blue}{X}                      & 3                     & \textcolor{blue}{X}                     & \textcolor{blue}{X}                      & 1                      \\ 
\hline
\textbf{Adbrain}                                 & \textcolor{blue}{X}                    & \textcolor{blue}{X}                      & 3                     & \textcolor{blue}{X}                     & \textcolor{blue}{X}                      & \textcolor{blue}{X}                     \\ 
\hline
\textbf{Vdopia}                                  & \textcolor{blue}{X}                    & \textcolor{blue}{X}                      & 3                     & \textcolor{blue}{X}                     & \textcolor{blue}{X}                      & \textcolor{blue}{X}                     \\ 
\hline
\textbf{Stripe}                                  & \textcolor{blue}{X}                    & \textcolor{blue}{X}                      & 10                    & \textcolor{blue}{X}                     & \textcolor{blue}{X}                      & 13                     \\ 
\hline
\textbf{Wingify}                                 & \textcolor{blue}{X}                    & \textcolor{blue}{X}                      & 7                     & \textcolor{blue}{X}                     & \textcolor{blue}{X}                      & 10                     \\ 
\hline
\textbf{BlueCava}                                & \textcolor{blue}{X}                    & \textcolor{blue}{X}                      & 1                     & \textcolor{blue}{X}                     & \textcolor{blue}{X}                      & \textcolor{blue}{X}                     \\ 
\hline
\textbf{Adara Media}                             & \textcolor{blue}{X}                    & \textcolor{blue}{X}                      & 5                     & \textcolor{blue}{X}                     & \textcolor{blue}{X}                      & \textcolor{blue}{X}                     \\ 
\hline
\textbf{Pinterest}                               & \textcolor{blue}{X}                    & \textcolor{blue}{X}                      & 2                     & \textcolor{blue}{X}                     & \textcolor{blue}{X}                      & 2                      \\ 
\hline
\textbf{RunAds}                                  & \textcolor{blue}{X}                    & \textcolor{blue}{X}                      & 6                     & \textcolor{blue}{X}                     & \textcolor{blue}{X}                      & \textcolor{blue}{X}                     \\ 
\hline
\textbf{Yandex}                                  & \textcolor{blue}{X}                    & \textcolor{blue}{X}                      & 7                     & \textcolor{blue}{X}                     & 7                       & 7                      \\ 
\hline
\textbf{CPMStar}                                 & \textcolor{blue}{X}                    & \textcolor{blue}{X}                      & 1                     & \textcolor{blue}{X}                     & \textcolor{blue}{X}                      & \textcolor{blue}{X}                     \\ 
\hline
\textbf{Gnezdo}                                  & \textcolor{blue}{X}                    & \textcolor{blue}{X}                      & 3                     & \textcolor{blue}{X}                     & \textcolor{blue}{X}                      & 3                      \\ 
\hline
\textbf{Permutive}                               & \textcolor{blue}{X}                    & \textcolor{blue}{X}                      & 2                     & 6                      & \textcolor{blue}{X}                      & 7                      \\ 
\hline
\textbf{DirectAdvert}                            & \textcolor{blue}{X}                    & \textcolor{blue}{X}                      & 3                     & \textcolor{blue}{X}                     & \textcolor{blue}{X}                      & \textcolor{blue}{X}                     \\ 
\hline
\textbf{DataMind.ru}   & \textcolor{blue}{X}                    & \textcolor{blue}{X}                      & 5                     & \textcolor{blue}{X}                     & \textcolor{blue}{X}                      & 3                      \\ 
\hline
\textbf{Sortable}                                & \textcolor{blue}{X}                    & \textcolor{blue}{X}                      & 1                     & 13                     & \textcolor{blue}{X}                      & \textcolor{blue}{X}                     \\ 
\hline
\textbf{Navegg}                                  & \textcolor{blue}{X}                    & \textcolor{blue}{X}                      & 2                     & \textcolor{blue}{X}                     & \textcolor{blue}{X}                      & \textcolor{blue}{X}                     \\ 
\hline
\textbf{Improve Digital}                         & \textcolor{blue}{X}                    & \textcolor{blue}{X}                      & 2                     & 7                      & 1                       & 7                      \\ 
\hline
\textbf{Yieldlab}                                & \textcolor{blue}{X}                    & \textcolor{blue}{X}                      & 2                     & 12                     & 2                       & 12                     \\ 
\hline
\textbf{SpotXchange}                             & \textcolor{blue}{X}                    & \textcolor{blue}{X}                      & 1                     & 1                      & 3                       & 1                      \\ 
\hline
\textbf{Rambler}                                 & \textcolor{blue}{X}                    & \textcolor{blue}{X}                      & 1                     & \textcolor{blue}{X}                     & \textcolor{blue}{X}                      & \textcolor{blue}{X}                     \\ 
\hline
\textbf{AdStir}                                  & \textcolor{blue}{X}                    & \textcolor{blue}{X}                      & 1                     & \textcolor{blue}{X}                     & \textcolor{blue}{X}                      & \textcolor{blue}{X}                     \\ 
\hline
\textbf{Adobe}                                   & \textcolor{blue}{X}                    & \textcolor{blue}{X}                      & \textcolor{blue}{X}                    & 1                      & 1                       & \textcolor{blue}{X}                     \\ 
\hline
\textbf{RubiconProject}                          & \textcolor{blue}{X}                    & \textcolor{blue}{X}                      & \textcolor{blue}{X}                    & 1                      & 1                       & \textcolor{blue}{X}                     \\ 
\hline
\textbf{Amobee}                                  & \textcolor{blue}{X}                    & \textcolor{blue}{X}                      & \textcolor{blue}{X}                    & 2                      & 3                       & \textcolor{blue}{X}                     \\ 
\hline
\textbf{Criteo}                                  & \textcolor{blue}{X}                    & \textcolor{blue}{X}                      & \textcolor{blue}{X}                    & 2                      & 1                       & \textcolor{blue}{X}                     \\ 
\hline
\textbf{Adelphic}                                & \textcolor{blue}{X}                    & \textcolor{blue}{X}                      & \textcolor{blue}{X}                    & 5                      & 7                       & 6                      \\ 
\hline
\textbf{Teads.tv}      & \textcolor{blue}{X}                    & \textcolor{blue}{X}                      & \textcolor{blue}{X}                    & 3                      & 3                       & 4                      \\ 
\hline
\textbf{INFOnline}                               & \textcolor{blue}{X}                    & \textcolor{blue}{X}                      & \textcolor{blue}{X}                    & 12                     & \textcolor{blue}{X}                      & 12                     \\ 
\hline
\textbf{Delta Projects}                          & \textcolor{blue}{X}                    & \textcolor{blue}{X}                      & \textcolor{blue}{X}                    & 6                      & 7                       & 6                      \\ 
\hline
\textbf{CBS Interactive}                         & \textcolor{blue}{X}                    & \textcolor{blue}{X}                      & \textcolor{blue}{X}                    & 15                     & \textcolor{blue}{X}                      & \textcolor{blue}{X}                     \\ 
\hline
\textbf{Cedexis}                                 & \textcolor{blue}{X}                    & \textcolor{blue}{X}                      & \textcolor{blue}{X}                    & 11                     & \textcolor{blue}{X}                      & \textcolor{blue}{X}                     \\ 
\hline
\textbf{RTBHouse}                                & \textcolor{blue}{X}                    & \textcolor{blue}{X}                      & \textcolor{blue}{X}                    & 11                     & \textcolor{blue}{X}                      & 9                      \\ 
\hline
\end{tabular}
\end{table*}

\begin{table*}
\centering
	\caption{The summary of bidders that did not appear before opt-out and appeared after opt-out in HTTP data, part 4}
	\label{tbl:in_test_not_in_train_4}
\begin{tabular}{|l|l|l|l|l|l|l|} 
\hline
\textbf{Advertiser/Bidders/3rd Party Service}                           & \textbf{Onetrust\_CA} & \textbf{~Cookiebot\_CA} & \textbf{~Central\_CA} & \textbf{~Onetrust\_GE} & \textbf{~Cookiebot\_GE} & \textbf{~Central\_GE}  \\ 
\hline
\textbf{VDX}                                     & \textcolor{blue}{X}                    & \textcolor{blue}{X}                      & \textcolor{blue}{X}                    & 4                      & 4                       & \textcolor{blue}{X}                     \\ 
\hline
\textbf{Gemius}                                  & \textcolor{blue}{X}                    & \textcolor{blue}{X}                      & \textcolor{blue}{X}                    & 14                     & 12                      & 4                      \\ 
\hline
\textbf{Gravity}                                 & \textcolor{blue}{X}                    & \textcolor{blue}{X}                      & \textcolor{blue}{X}                    & 2                      & \textcolor{blue}{X}                      & \textcolor{blue}{X}                     \\ 
\hline
\textbf{Nativo}                                  & \textcolor{blue}{X}                    & \textcolor{blue}{X}                      & \textcolor{blue}{X}                    & 5                      & \textcolor{blue}{X}                      & \textcolor{blue}{X}                     \\ 
\hline
\textbf{StackAdapt}                              & \textcolor{blue}{X}                    & \textcolor{blue}{X}                      & \textcolor{blue}{X}                    & 8                      & 7                       & 9                      \\ 
\hline
\textbf{TripleLift}                              & \textcolor{blue}{X}                    & \textcolor{blue}{X}                      & \textcolor{blue}{X}                    & 4                      & \textcolor{blue}{X}                      & 2                      \\ 
\hline
\textbf{LiveIntent}                              & \textcolor{blue}{X}                    & \textcolor{blue}{X}                      & \textcolor{blue}{X}                    & 1                      & 2                       & 1                      \\ 
\hline
\textbf{Taboola}                                 & \textcolor{blue}{X}                    & \textcolor{blue}{X}                      & \textcolor{blue}{X}                    & 2                      & 2                       & \textcolor{blue}{X}                     \\ 
\hline
\textbf{Rhythm}                                  & \textcolor{blue}{X}                    & \textcolor{blue}{X}                      & \textcolor{blue}{X}                    & 4                      & 3                       & \textcolor{blue}{X}                     \\ 
\hline
\textbf{Admedo}                                  & \textcolor{blue}{X}                    & \textcolor{blue}{X}                      & \textcolor{blue}{X}                    & 2                      & 1                       & 14                     \\ 
\hline
\textbf{Datonics}                                & \textcolor{blue}{X}                    & \textcolor{blue}{X}                      & \textcolor{blue}{X}                    & 1                      & \textcolor{blue}{X}                      & \textcolor{blue}{X}                     \\ 
\hline
\textbf{Eyeota}                                  & \textcolor{blue}{X}                    & \textcolor{blue}{X}                      & \textcolor{blue}{X}                    & 1                      & \textcolor{blue}{X}                      & \textcolor{blue}{X}                     \\ 
\hline
\textbf{Tchibo}                                  & \textcolor{blue}{X}                    & \textcolor{blue}{X}                      & \textcolor{blue}{X}                    & 1                      & \textcolor{blue}{X}                      & 2                      \\ 
\hline
\textbf{ConversantMedia}                         & \textcolor{blue}{X}                    & \textcolor{blue}{X}                      & \textcolor{blue}{X}                    & 2                      & 2                       & 1                      \\ 
\hline
\textbf{MediaMath}                               & \textcolor{blue}{X}                    & \textcolor{blue}{X}                      & \textcolor{blue}{X}                    & 1                      & 1                       & \textcolor{blue}{X}                     \\ 
\hline
\textbf{RoqAd}                                   & \textcolor{blue}{X}                    & \textcolor{blue}{X}                      & \textcolor{blue}{X}                    & 1                      & 1                       & 7                      \\ 
\hline
\textbf{TheReachGroup}                           & \textcolor{blue}{X}                    & \textcolor{blue}{X}                      & \textcolor{blue}{X}                    & \textcolor{blue}{X}                     & 3                       & 5                      \\ 
\hline
\textbf{OpenX}                                   & \textcolor{blue}{X}                    & \textcolor{blue}{X}                      & \textcolor{blue}{X}                    & \textcolor{blue}{X}                     & 1                       & \textcolor{blue}{X}                     \\ 
\hline
\textbf{MobFox}                                  & \textcolor{blue}{X}                    & \textcolor{blue}{X}                      & \textcolor{blue}{X}                    & \textcolor{blue}{X}                     & \textcolor{blue}{X}                      & 14                     \\ 
\hline
\textbf{NanoInteractive}                         & \textcolor{blue}{X}                    & \textcolor{blue}{X}                      & \textcolor{blue}{X}                    & \textcolor{blue}{X}                     & \textcolor{blue}{X}                      & 16                     \\ 
\hline
\textbf{Avocet}                                  & \textcolor{blue}{X}                    & \textcolor{blue}{X}                      & \textcolor{blue}{X}                    & \textcolor{blue}{X}                     & \textcolor{blue}{X}                      & 11                     \\ 
\hline
\textbf{Hurra.com}    & \textcolor{blue}{X}                    & \textcolor{blue}{X}                      & \textcolor{blue}{X}                    & \textcolor{blue}{X}                     & \textcolor{blue}{X}                      & 4                      \\ 
\hline
\textbf{AdSpirit}                                & \textcolor{blue}{X}                    & \textcolor{blue}{X}                      & \textcolor{blue}{X}                    & \textcolor{blue}{X}                     & \textcolor{blue}{X}                      & 2                      \\ 
\hline
\textbf{GENIEE}                                  & \textcolor{blue}{X}                    & \textcolor{blue}{X}                      & \textcolor{blue}{X}                    & \textcolor{blue}{X}                     & \textcolor{blue}{X}                      & 1                      \\ 
\hline
\textbf{AdTelligent}                             & \textcolor{blue}{X}                    & \textcolor{blue}{X}                      & \textcolor{blue}{X}                    & \textcolor{blue}{X}                     & \textcolor{blue}{X}                      & 3                      \\ 
\hline
\textbf{BidSwitch}                               & \textcolor{blue}{X}                    & \textcolor{blue}{X}                      & \textcolor{blue}{X}                    & \textcolor{blue}{X}                     & \textcolor{blue}{X}                      & 1                      \\ 
\hline
\textbf{Digital Target}                          & \textcolor{blue}{X}                    & \textcolor{blue}{X}                      & \textcolor{blue}{X}                    & 0                      & 0                       & 1                      \\
\hline
\end{tabular}
\end{table*}

\textcolor{blue}{In this analysis, we first exacted the advertisers/bidders/3rd party service list from the HTTP data before and after opt-out, and filtered the ones that appeared after opt-out and did not appear before opt-out. The results are included into Table \ref{tbl:in_test_not_in_train_1} to Table \ref{tbl:in_test_not_in_train_4}. The first column is the name of advertisers, bidders, or other third party service names. The number in specific column represents the number of personas (total number of personas is 16). Blue \textbf{X} represents this advertiser, bidder, or other third party service did not meet the analysis condition: "appeared after opt-out and did not appear before opt-out" in the current CMP-IP setting.}

\textcolor{blue}{The purpose of this analysis is figure out which bidders violate the opt-out, especially did the ``selling personal information''. So we compared the bidders in HTTP data and the bidders in bids dataset. From the HTTP bidder dataset, we have the advertiser/bidder/3rd party service list that appeared after opt-out and disappeared before opt-out. From the bids dataset, we have the bidder list that appeared after opt-out, and the bids value is 10 percent larger than the same bidder in Control. The intersection of bidder list between the bidder list in HTTP bidder dataset and in bids dataset, we have the results displayed in Table \ref{tbl:in_test_not_in_train}. However, the bidder \textbf{SmartAdServer} and \textbf{Teads.tv} are all in setting Central opt-out, and those 2 bidders are not listed into the Central opt-out website \cite{nai_opt_out}. So in this analysis, we do not obtain a bidder list that violate the regulation and reselling personal information.}
