# Supplementary material for: Opted Out, Yet Tracked: Are Regulations Enough to Protect Your Privacy?
Source: arXiv:2202.00885 source file (2023-10-06)
Supplement: Supplementary file 2 [file 7_appendix.tex]

\begin{table*}[!h]
%\adjustbox{max width=\textwidth}{
    \centering
        \caption{Ad bidding under GDPR in France. Avg. column represents the mean of all bid value. Std. represents the standard deviation of all bid value. Opt-out and opt-in represent the bids when we opt-out and opt-in the selling of user data, respectively.  $\uparrow$ and $\downarrow$ indicate bid values that are higher and lower than Control's avg., respectively. $\textcolor{red}{\uparrow}$ and $\textcolor{red}{\downarrow}$ indicate bid values that are Control's avg. $\pm$ std., respectively.}
    \begin{tabular}{l?{0.3mm}rr|rr?{0.3mm}rr|rr?{0.3mm}rr|rr} 
    \toprule
     & \multicolumn{4}{c?{0.3mm}}{\textbf{OneTrust}} & \multicolumn{4}{c?{0.3mm}}{\textbf{CookieBot}}& \multicolumn{4}{c}{\textbf{NAI}}    \\ 
     & \multicolumn{2}{c}{\textbf{Opt-out}}& \multicolumn{2}{c?{0.3mm}}{\textbf{Opt-in}}     & \multicolumn{2}{c}{\textbf{Opt-out}}& \multicolumn{2}{c?{0.3mm}}{\textbf{Opt-in}}    & \multicolumn{2}{c}{\textbf{Opt-out}}& \multicolumn{2}{c}{\textbf{Opt-in}}   \\ 
    \textbf{Persona}     & \multicolumn{1}{c}{\textbf{Avg.}} & \multicolumn{1}{c|}{\textbf{Std.}} & \multicolumn{1}{c}{\textbf{Avg.}} & \multicolumn{1}{c?{0.3mm}}{\textbf{Std.}} & \multicolumn{1}{c}{\textbf{Avg.}} & \multicolumn{1}{c|}{\textbf{Std.}} & \multicolumn{1}{c}{\textbf{Avg.}} & \multicolumn{1}{c?{0.3mm}}{\textbf{Std.}}  & \multicolumn{1}{c}{\textbf{Avg.}} & \multicolumn{1}{c|}{\textbf{Std.}} & \multicolumn{1}{c}{\textbf{Avg.}} & \multicolumn{1}{c}{\textbf{Std.}}  \\ 
    \toprule

    \textbf{Adult}                                                              & 0.21$^{\uparrow}$                                           & 0.21                                          & 0.16$^{\downarrow}$                                          & 0.16                                                                                   & 0.10$^{\uparrow}$                                           & 0.00                                          & 0.02$^{\downarrow}$                                          & 0.01                                                                                  & 0.31$^{\uparrow}$                                           & 0.32                                          & 0.19$^{\uparrow}$                                           & 0.18                                           \\ 
    
    \textbf{Arts}                                                               & 0.05$^{\downarrow}$                                          & 0.07                                          & 0.50$^{\uparrow}$                                           & 0.45                                                                                    & 0.04$^{\downarrow}$                                          & 0.03                                          & 0.03$^{\downarrow}$                                          & 0.05                                           & 0.29$^{\uparrow}$                                           & 0.17                                          & 0.24$^{\textcolor{red}{\uparrow}}$                                           & 0.17                                           \\ 
    
    \textbf{Business}                                                           & 0.03$^{\downarrow}$                                          & 0.05                                          & 0.56$^{\uparrow}$                                           & 0.50                                           & 0.27$^{\textcolor{red}{\uparrow}}$                                           & 0.16                                          & 0.17$^{\uparrow}$                                           & 0.17                                           & 0.03$^{\textcolor{red}{\downarrow}}$                                          & 0.02                                          & 0.03$^{\textcolor{red}{\downarrow}}$                                          & 0.01                                           \\ 
    
    \textbf{Computers}                                                          & 0.33$^{\uparrow}$                                           & 0.52                                          & 0.67$^{\uparrow}$                                           & 0.88                                           & 0.23$^{\textcolor{red}{\uparrow}}$                                           & 0.12                                          & 0.11$^{\uparrow}$                                           & 0.07                                                                                    & 0.08$^{\textcolor{red}{\downarrow}}$                                          & 0.08                                          & 0.34$^{\textcolor{red}{\uparrow}}$                                           & 0.46                                           \\ 
    
    \textbf{Games}                                                              & 0.25$^{\uparrow}$                                          & 0.20                                          & 0.96$^{\uparrow}$                                          & 0.92                                                                                  & 0.21$^{\textcolor{red}{\uparrow}}$                                          & 0.22                                          & 0.20$^{\uparrow}$                                          & 0.23                                           & 0.13$^{\downarrow}$                                          & 0.15                                          & - & -  \\ 
    
    \textbf{Health}                                                             & 0.33$^{\uparrow}$                                          & 0.34                                          & 0.74$^{\uparrow}$                                          & 0.55                                                                                    & 0.28$^{\textcolor{red}{\uparrow}}$                                          & 0.41                                          & 0.32$^{\textcolor{red}{\uparrow}}$                                          & 0.18                                                                                   & - & - & - & -  \\ 
    
    \textbf{Home}                                                               & 0.30$^{\uparrow}$                                          & 0.40                                          & 0.85$^{\uparrow}$                                          & 1.28                                                                                    & 0.03$^{\downarrow}$                                          & 0.02                                          & 0.03$^{\downarrow}$                                          & 0.02                                           & 0.07$^{\textcolor{red}{\downarrow}}$                                          & 0.05                                          & 0.04$^{\textcolor{red}{\downarrow}}$                                          & 0.02                                           \\ 
    
    \textbf{Kids}                                                               & 0.33$^{\uparrow}$                                          & 0.34                                          & 0.54$^{\uparrow}$                                          & 0.76                                                                                    & 0.31$^{\textcolor{red}{\uparrow}}$                                          & 0.15                                          & 0.05$^{\downarrow}$                                          & 0.06                                                                                   & 0.14$^{\downarrow}$                                          & 0.18                                          & 0.17$^{\uparrow}$                                          & 0.45                                           \\ 
    
    \textbf{News}                                                               & 0.17$^{\downarrow}$                                          & 0.19                                          & 0.41$^{\downarrow}$                                          & 0.72                                           & 0.26$^{\textcolor{red}{\uparrow}}$                                          & 0.22                                          & 0.31$^{\textcolor{red}{\uparrow}}$                                          & 0.19                                                                                    & 0.07$^{\textcolor{red}{\downarrow}}$                                          & 0.05                                          & 0.05$^{\textcolor{red}{\downarrow}}$                                          & 0.04                                           \\ 
    
    \textbf{Recreation}                                                         & 0.23$^{\uparrow}$                                          & 0.22                                          & 0.22$^{\downarrow}$                                          & 0.27                                           & 0.33$^{\textcolor{red}{\uparrow}}$                                          & 0.18                                          & 0.06$^{\downarrow}$                                          & 0.00                                                                                    & 0.02$^{\textcolor{red}{\downarrow}}$                                          & 0.02                                          & 0.01$^{\textcolor{red}{\downarrow}}$                                          & 0.01                                           \\ 
    
    \textbf{Reference}                                                          & 0.29$^{\uparrow}$                                          & 0.18                                          & 0.68$^{\uparrow}$                                          & 0.86                                                                                    & 0.08$^{\downarrow}$                                          & 0.14                                          & 0.14$^{\uparrow}$                                          & 0.20                                                                                   & 0.24$^{\uparrow}$                                          & 0.18                                          & 0.23$^{\uparrow}$                                          & 0.15                                           \\ 
    
    \textbf{Regional}                                                           & 0.08$^{\downarrow}$                                          & 0.12                                          & 0.65$^{\uparrow}$                                          & 0.54                                                                                    & 0.14$^{\uparrow}$                                          & 0.19                                          & 0.04$^{\downarrow}$                                          & 0.03                                           & 0.30$^{\uparrow}$                                          & 0.29                                          & 0.21$^{\uparrow}$                                          & 0.15                                           \\ 
    
    \textbf{Science}                                                            & 0.21$^{\uparrow}$                                          & 0.22                                          & 0.77$^{\uparrow}$                                          & 1.13                                                                                    & 0.09$^{\downarrow}$                                          & 0.08                                          & 0.09$^{\downarrow}$                                          & 0.08                                           & 0.05$^{\textcolor{red}{\downarrow}}$                                          & 0.03                                          & 0.04$^{\textcolor{red}{\downarrow}}$                                          & 0.03                                           \\ 
    
    \textbf{Shopping}                                                           & 0.38$^{\textcolor{red}{\uparrow}}$                                          & 0.56                                          & 0.67$^{\uparrow}$                                          & 1.10                                           & 0.19$^{\textcolor{red}{\uparrow}}$                                          & 0.07                                          & 0.27$^{\textcolor{red}{\uparrow}}$                                          & 0.13                                                                                    & 0.07$^{\textcolor{red}{\downarrow}}$                                          & 0.15                                          & 0.34$^{\textcolor{red}{\uparrow}}$                                          & 0.68                                           \\ 
    
    \textbf{Society}                                                            & 0.34$^{\uparrow}$                                          & 0.36                                          & 0.50$^{\uparrow}$                                          & 0.63                                           & 0.27$^{\textcolor{red}{\uparrow}}$                                          & 0.26                                          & 0.19$^{\uparrow}$                                          & 0.19                                                                                    & 0.07$^{\textcolor{red}{\downarrow}}$                                          & 0.07                                          & 0.05$^{\textcolor{red}{\downarrow}}$                                          & 0.04                                           \\ 
    
    \textbf{Sports}                                                             & 0.48$^{\textcolor{red}{\uparrow}}$                                          & 0.38                                          & 0.80$^{\uparrow}$                                          & 0.99                                                                                   & 0.01$^{\textcolor{red}{\downarrow}}$                                          & 0.00                                          & 0.02$^{\downarrow}$                                          & 0.00                                           & 0.09$^{\downarrow}$                                          & 0.09                                          & 0.08$^{\textcolor{red}{\downarrow}}$                                          & 0.12                                           \\ 
    
    \midrule
    \textbf{Control}                                                            & 0.18                                          & 0.18                                          & 0.42                                          & 0.63                                                                                    & 0.09                                          & 0.07                                          & 0.09                                          & 0.15                                          &  0.22                                          & 0.14                                          & 0.16                                          & 0.07                                           \\
    
        \bottomrule
    
    \end{tabular}

    \label{table:GDPR-bidding-France-mean}
    \end{table*}
    
%\begin{appendices}
\appendix
\section{Appendix: Advertisers bidding behavior under GDPR}
\label{sec:appendix}

In this Appendix section, we present advertisers' average bidding under GDPR regulation in France for three iterations which is Table \ref{table:GDPR-bidding-France-mean}.

In Onetrust, when we opt-out, 12 personas receive higher bids than control, and 2 of them receive higher bids than the sum of control and the standard deviation of control.

In Cookiebot, 11 personas receive higher bids than control when we do the opt-out, and 9 of them even receive higher bids than the sum of control and the standard deviation of control.
%\end{appendices}
